# Supplementary material for: Sustaining star formation rates in spiral galaxies - Supernova-driven turbulent accretion disk models applied to THINGS galaxies
Source: arXiv:1009.3722 ancillary file (2010-09-20)

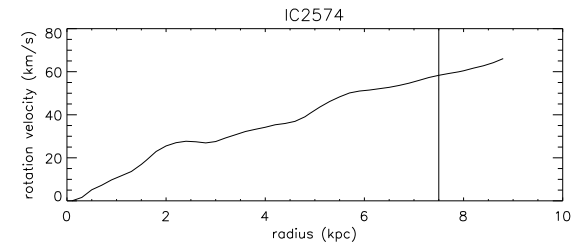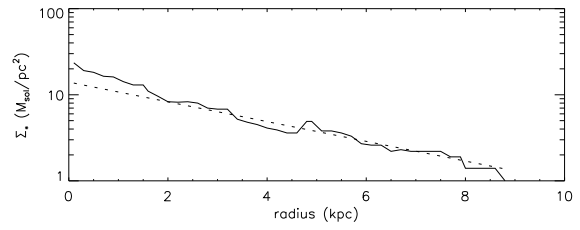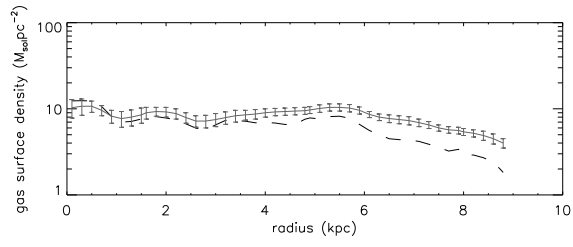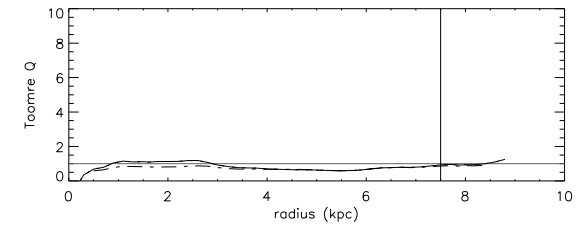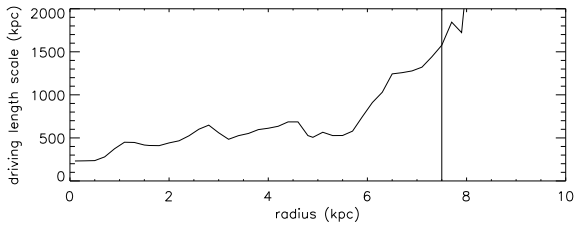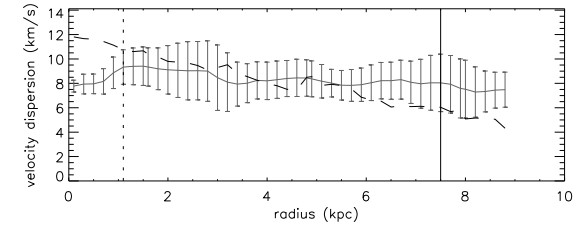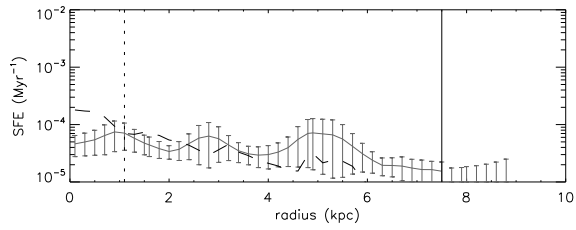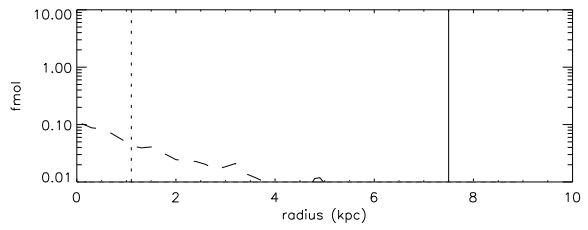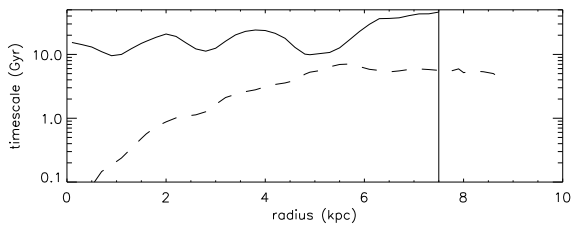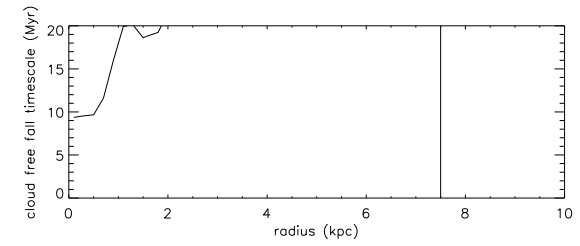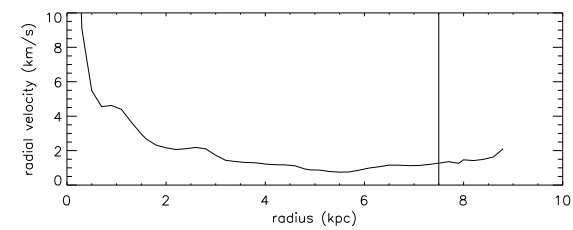

NGC4214

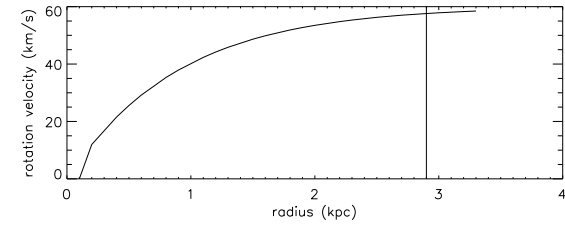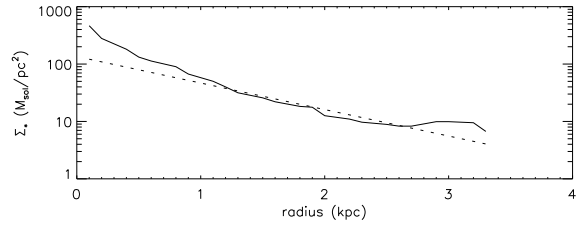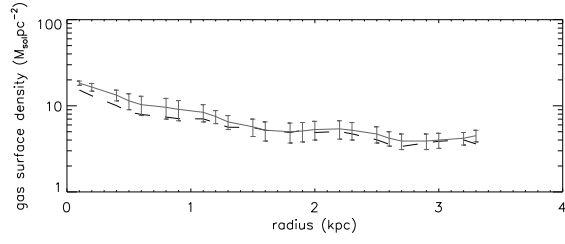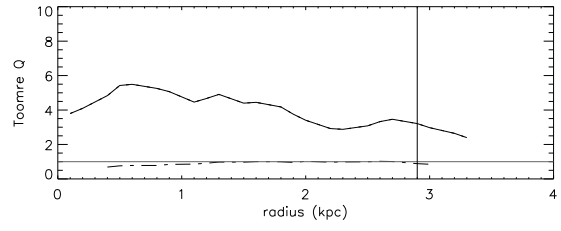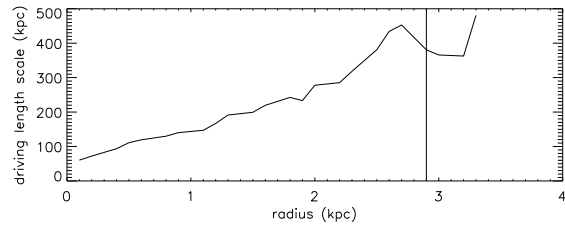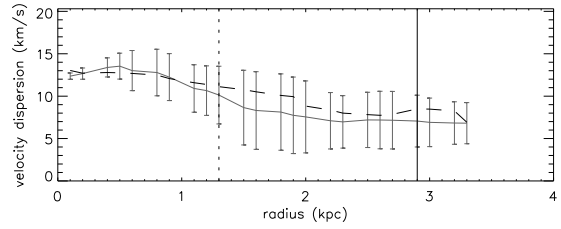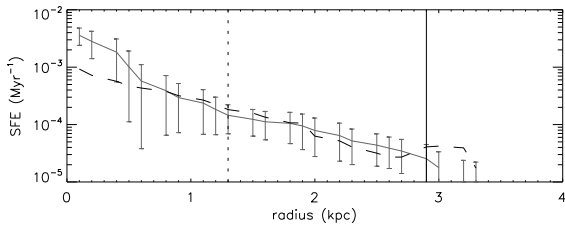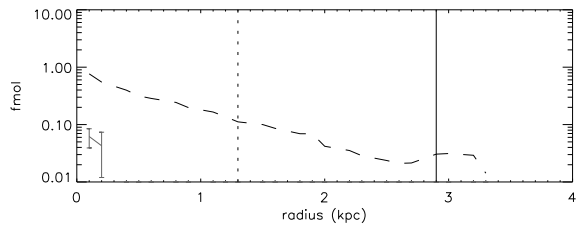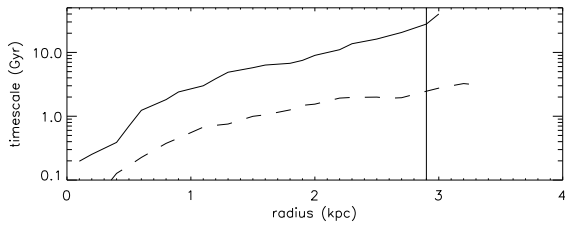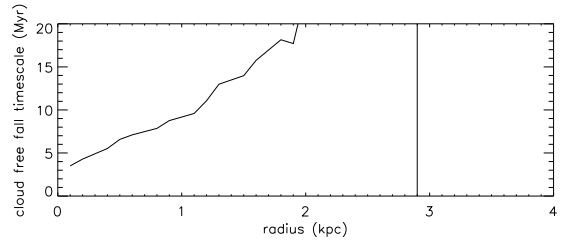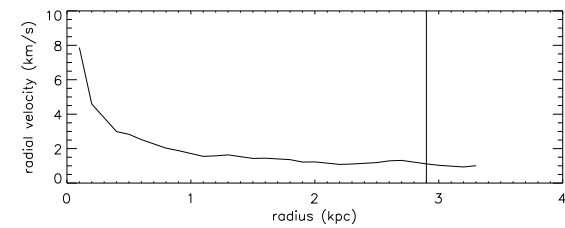

NGC2976

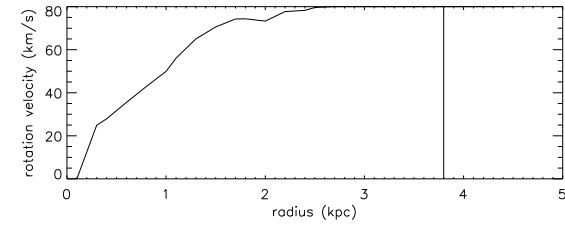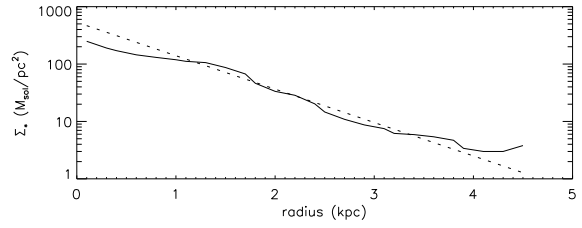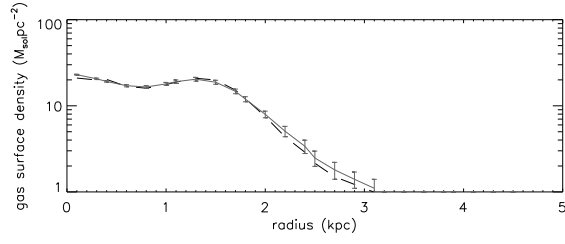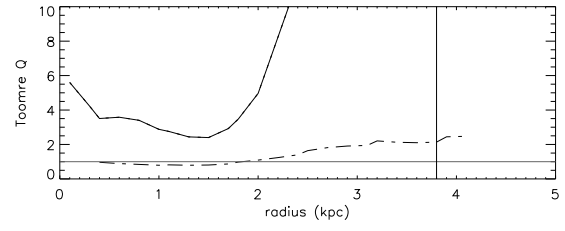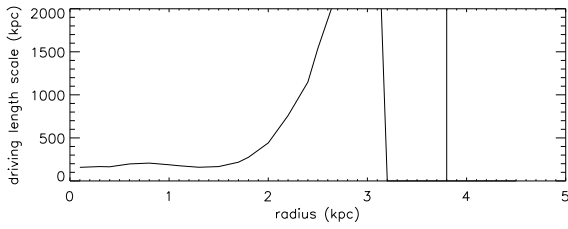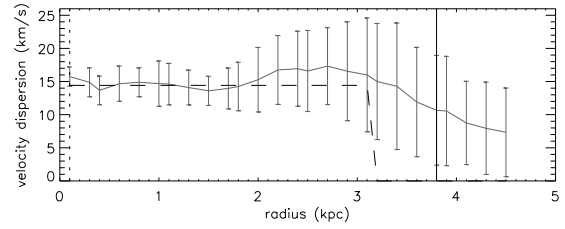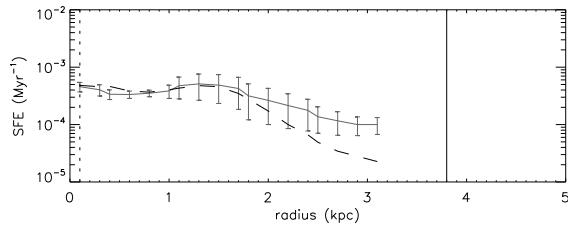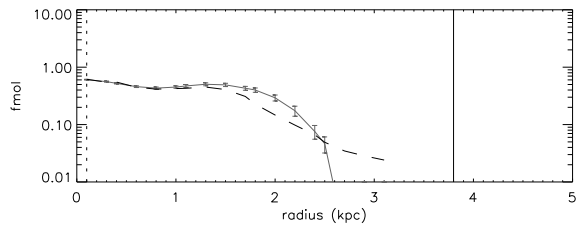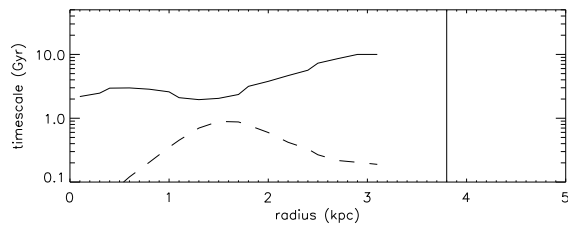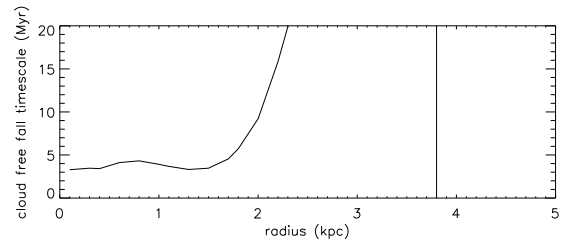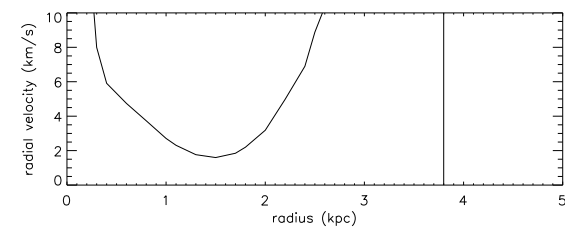

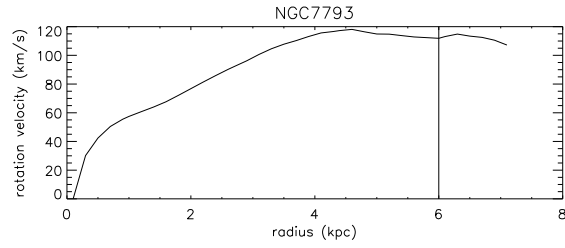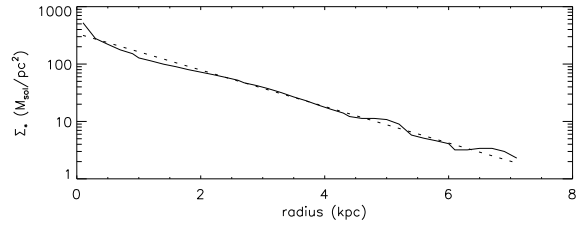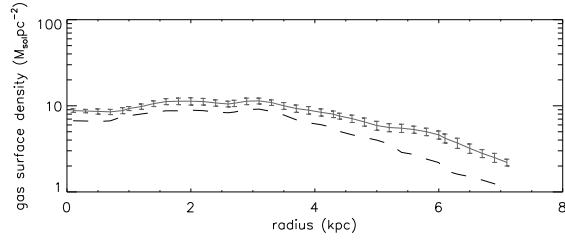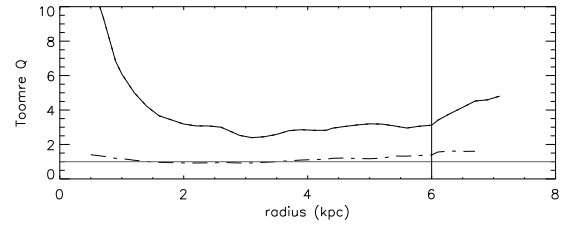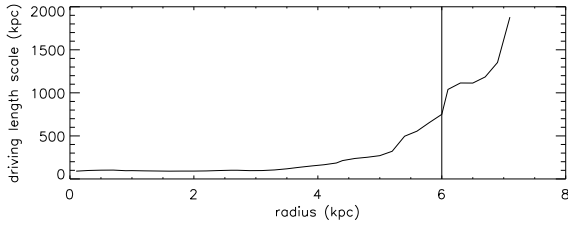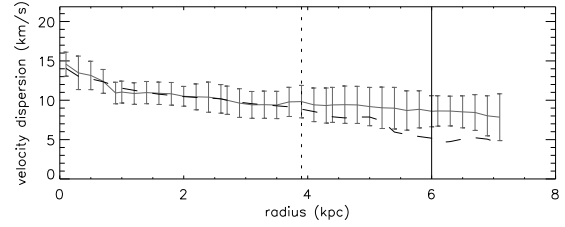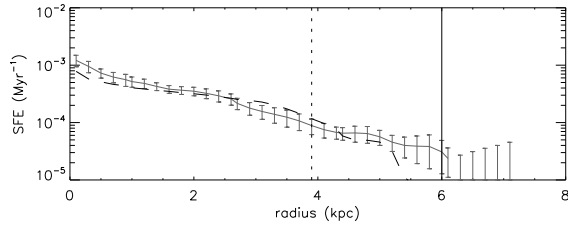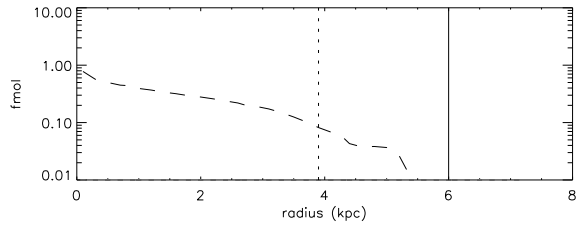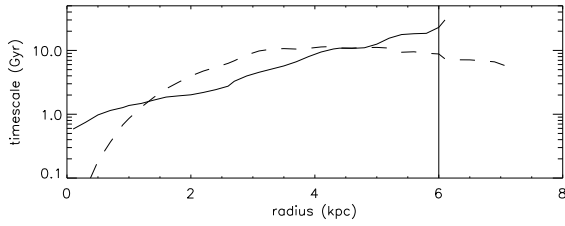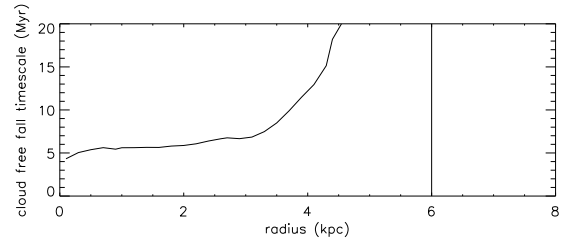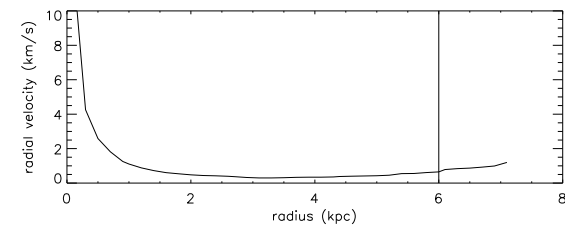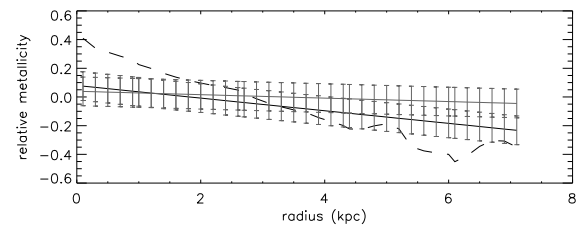

NGC2403

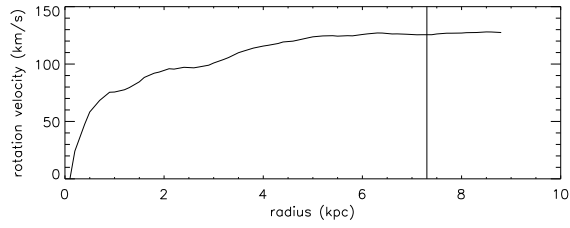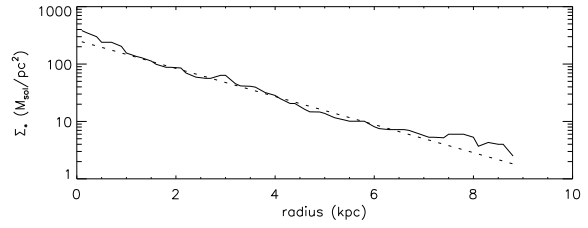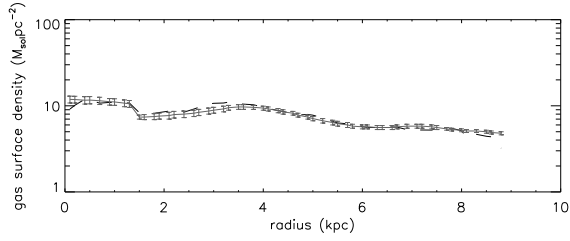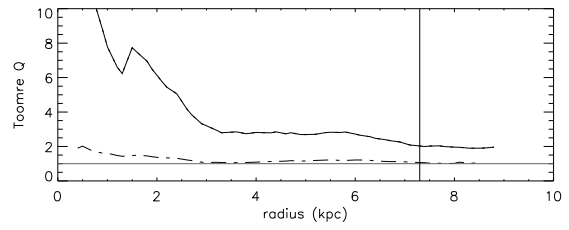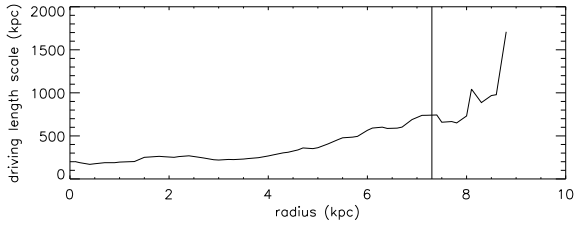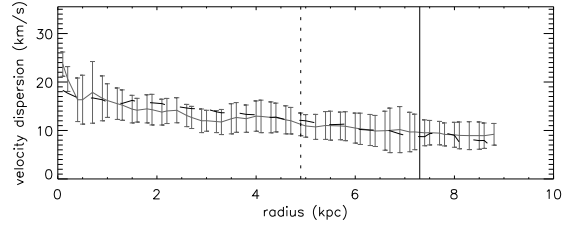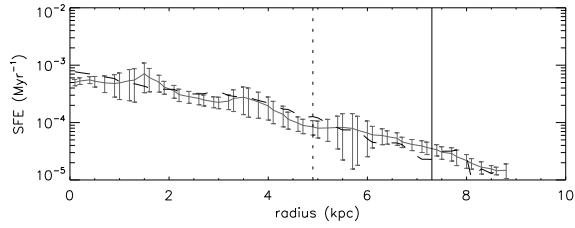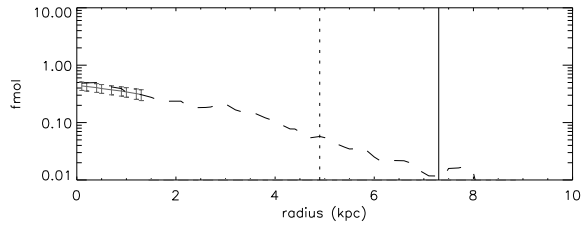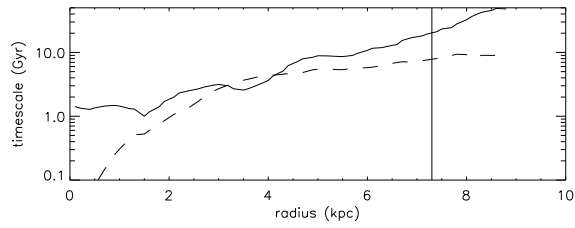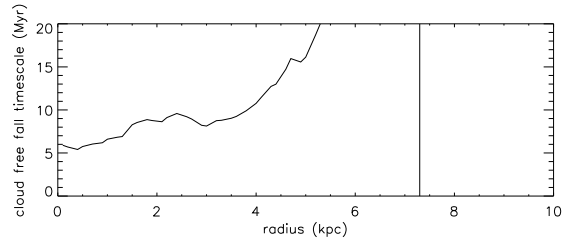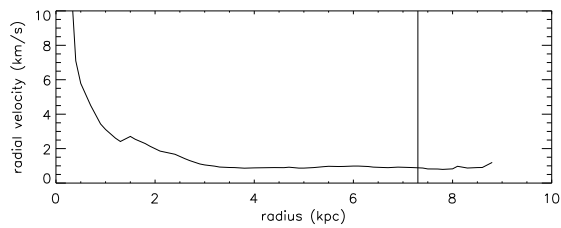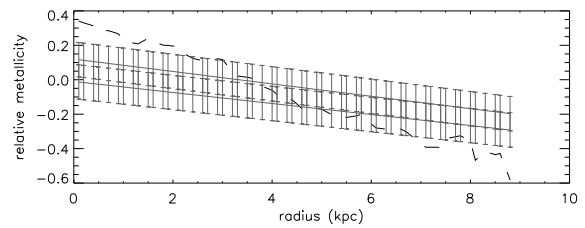

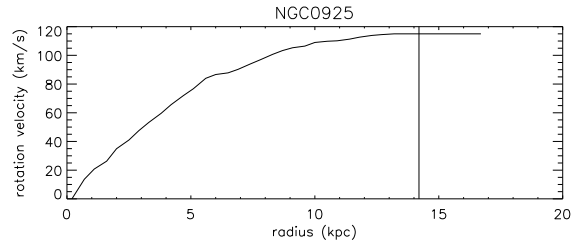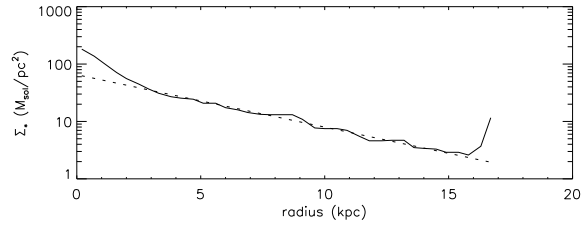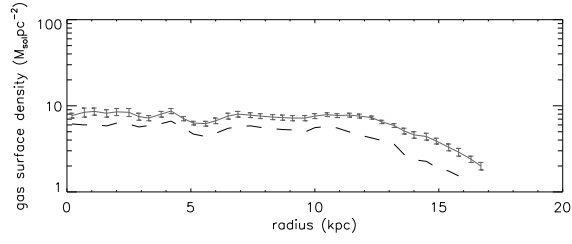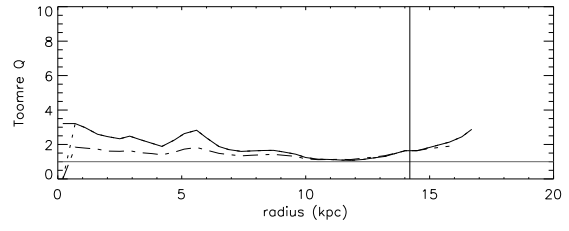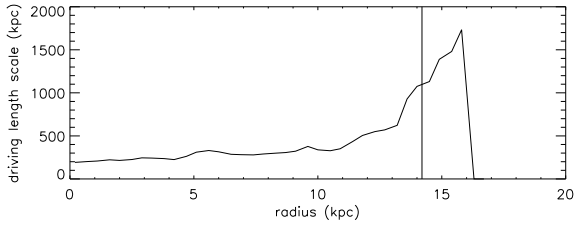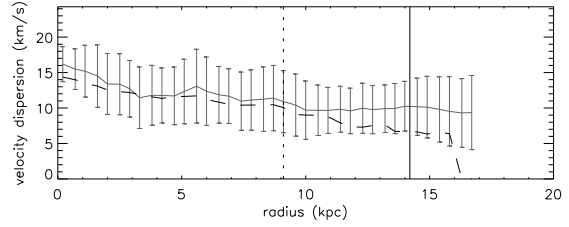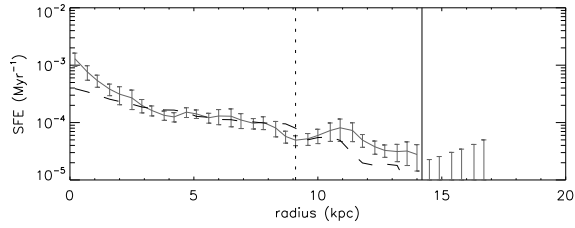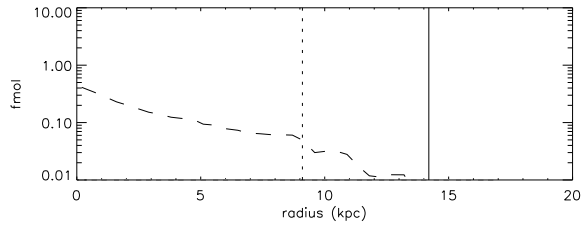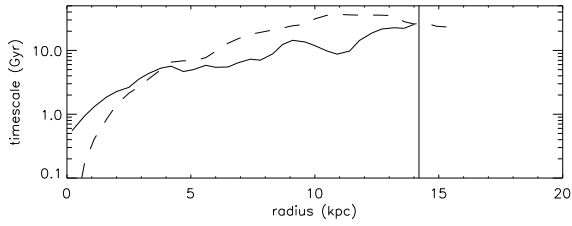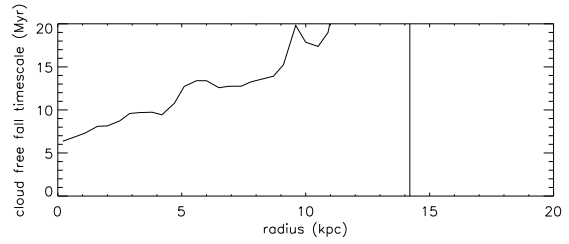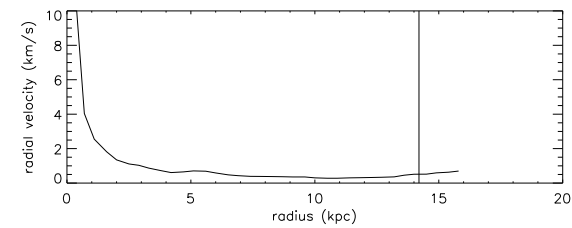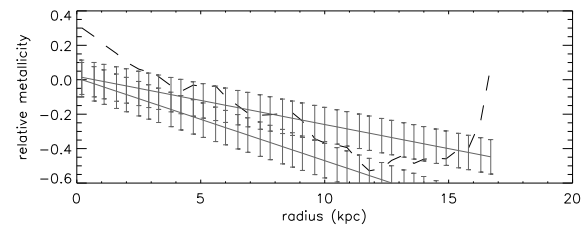

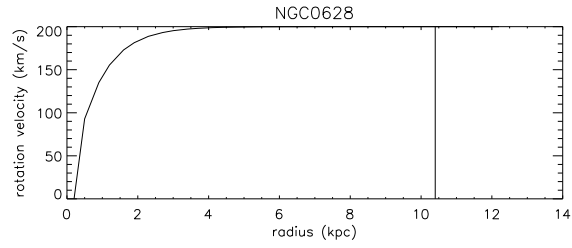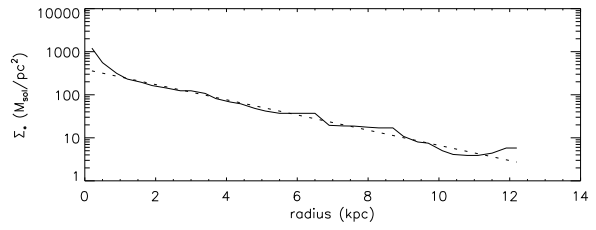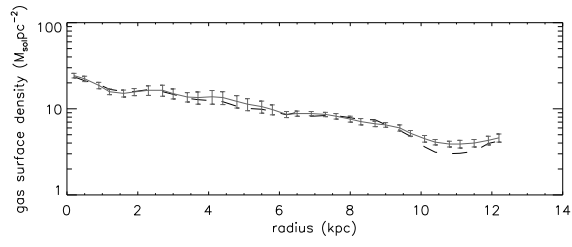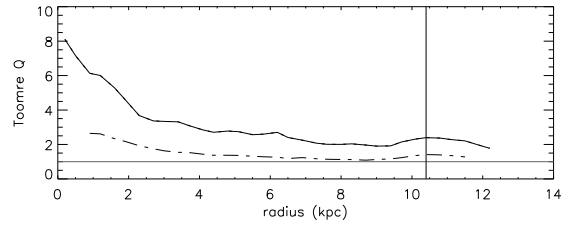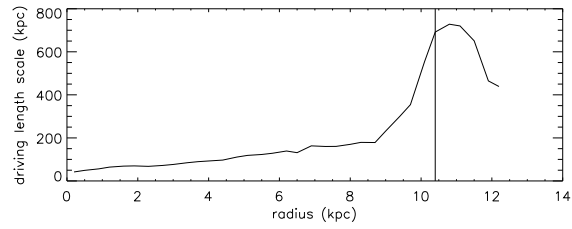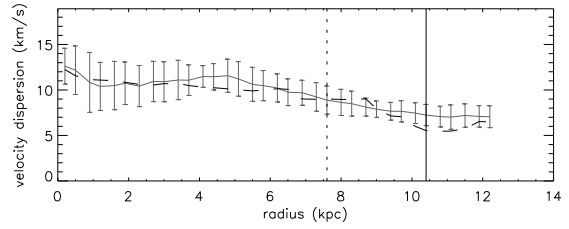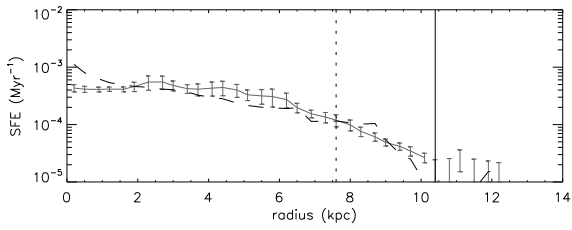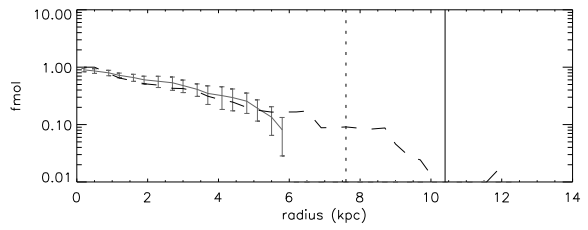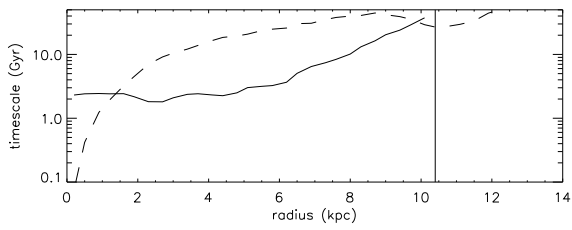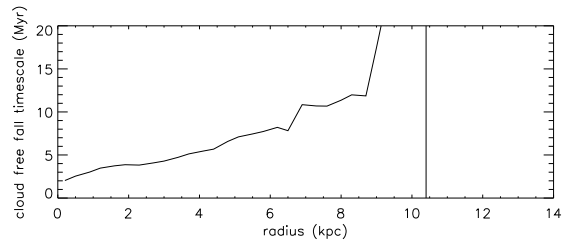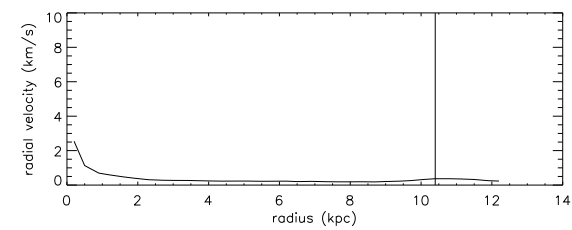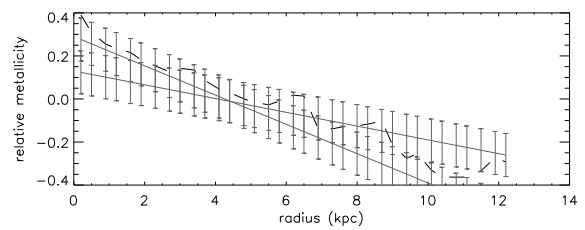

NGC3198

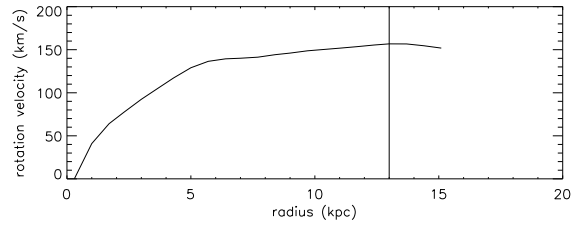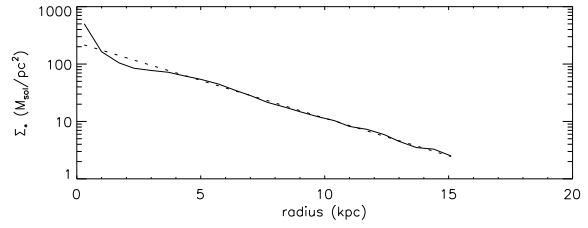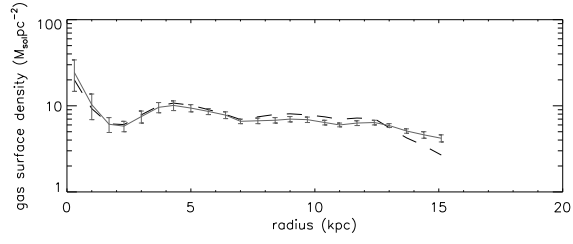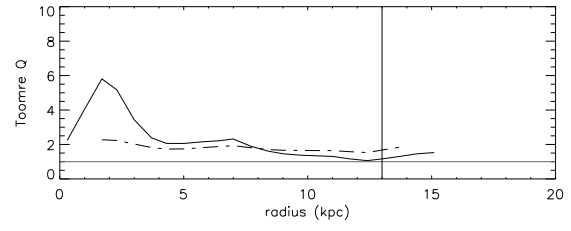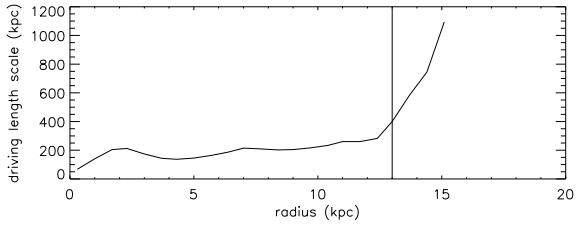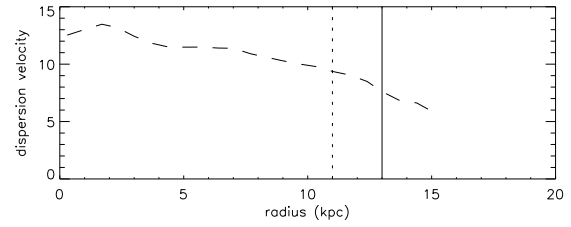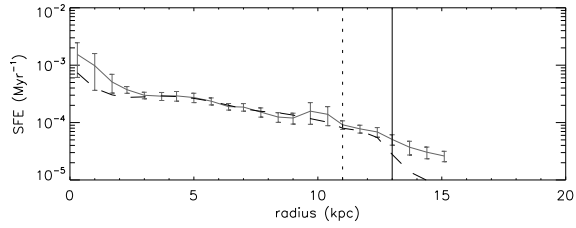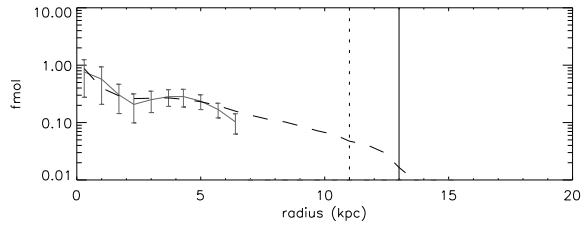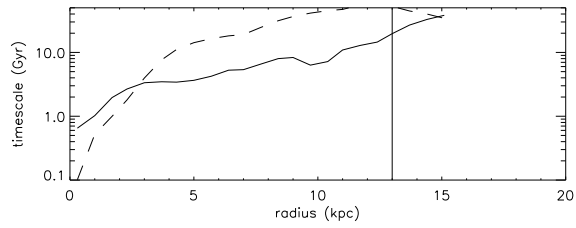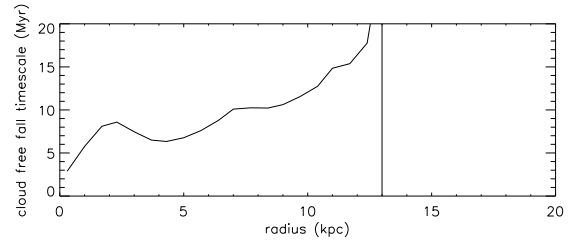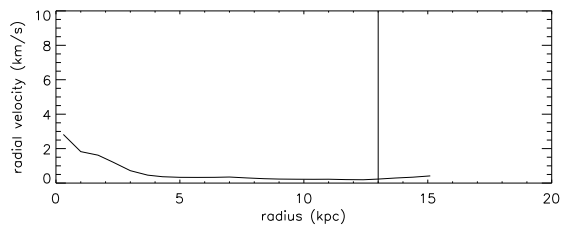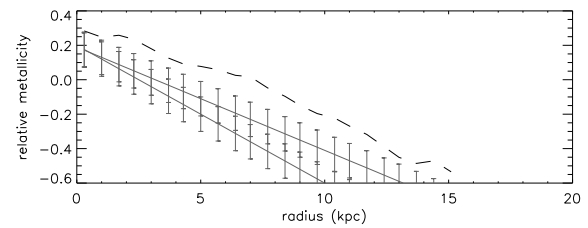



NGC3184

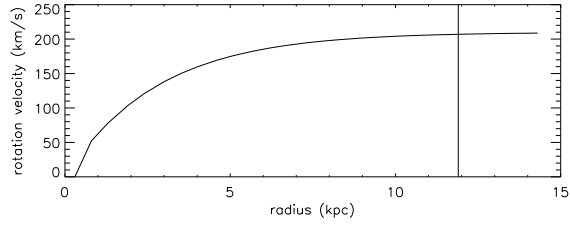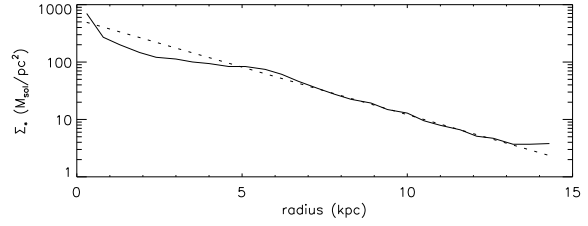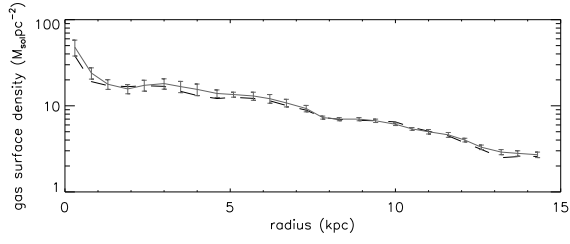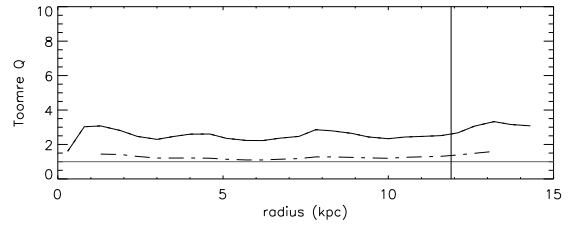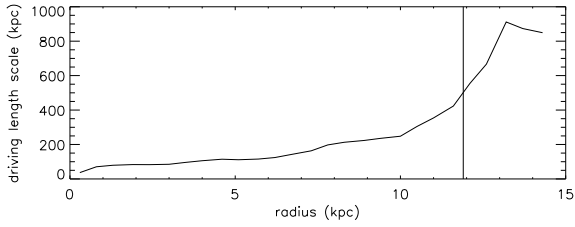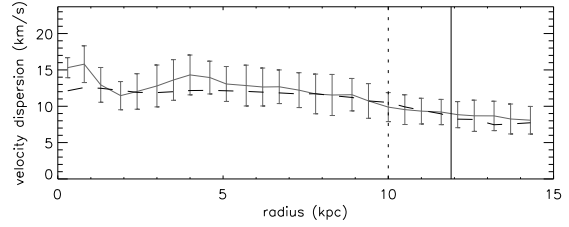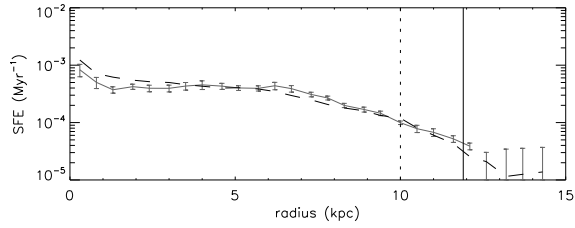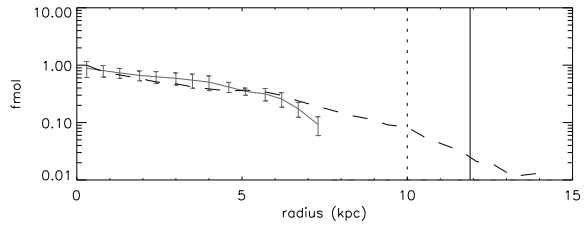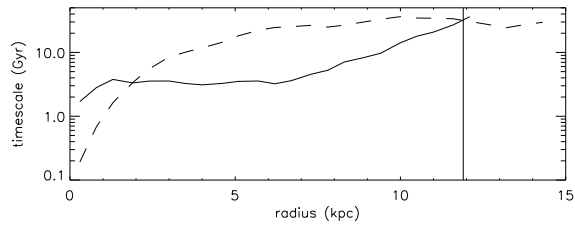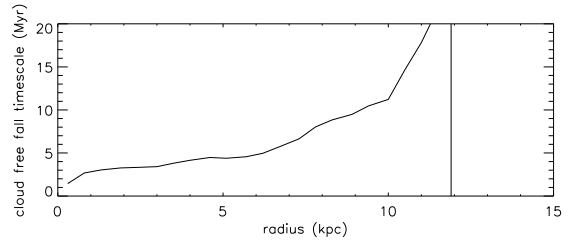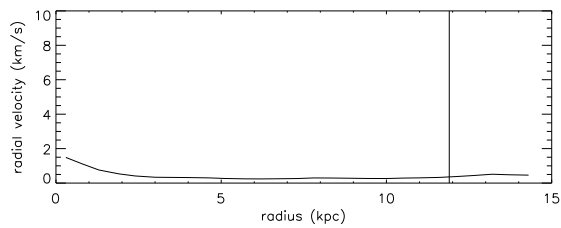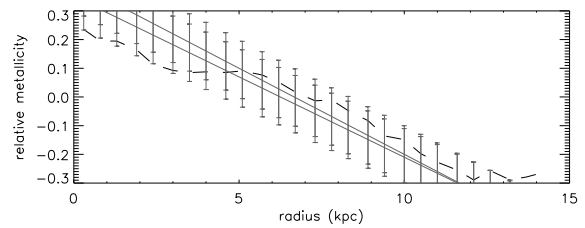

NGC4736

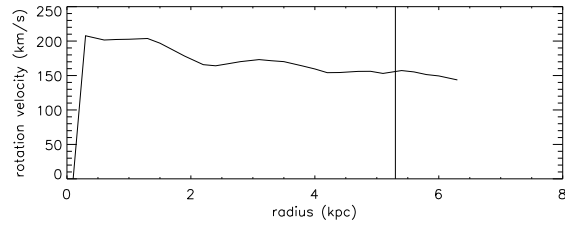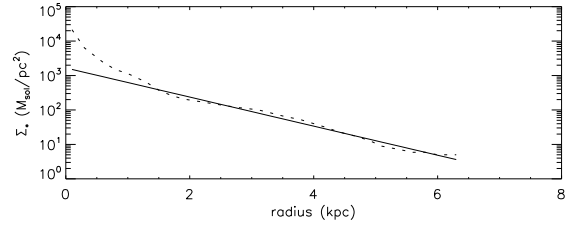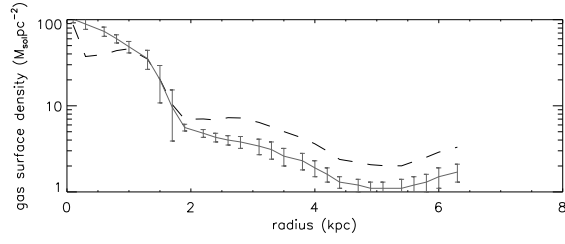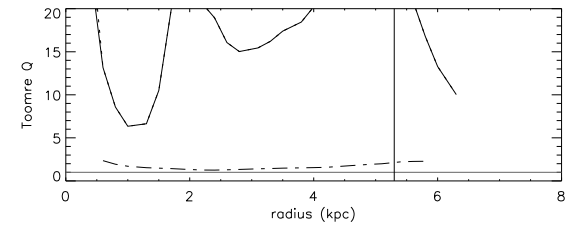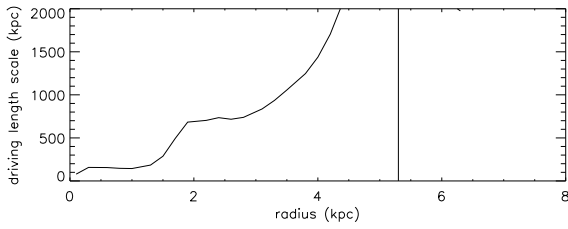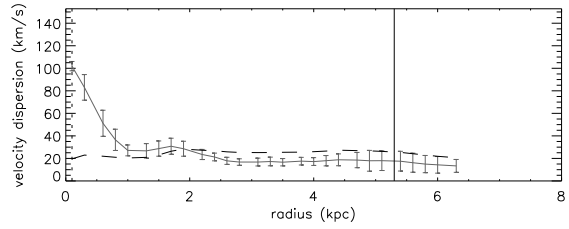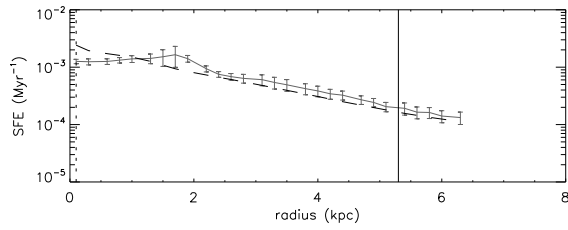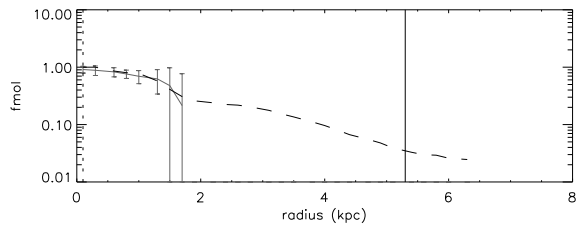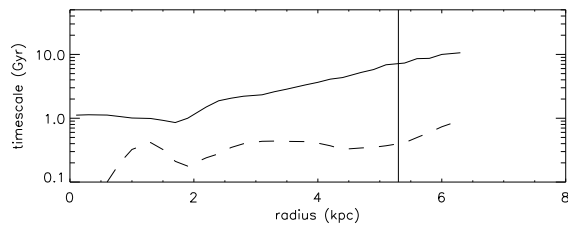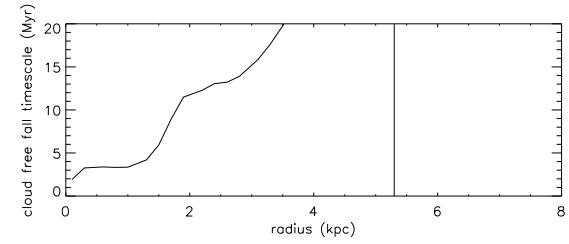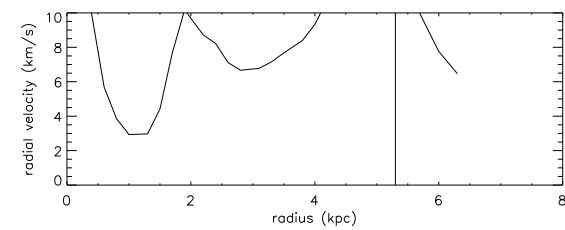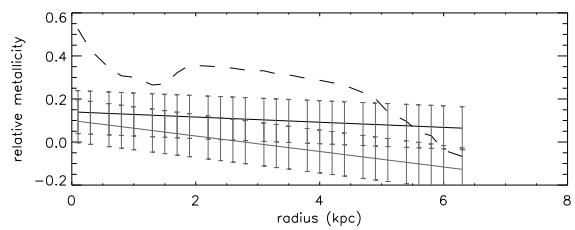

NGC 3351

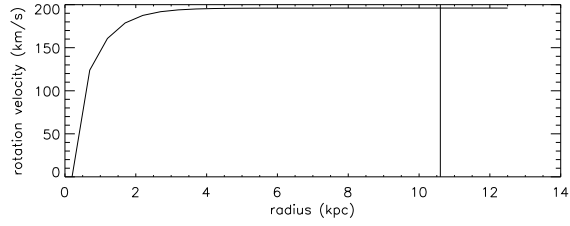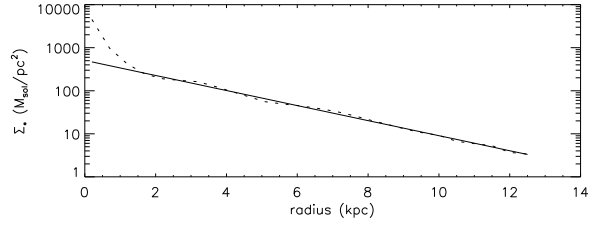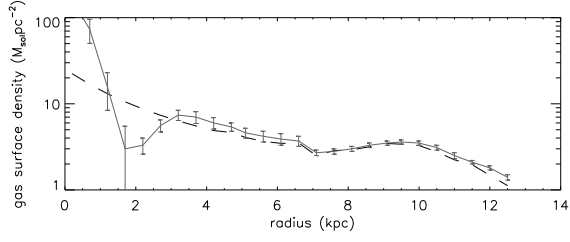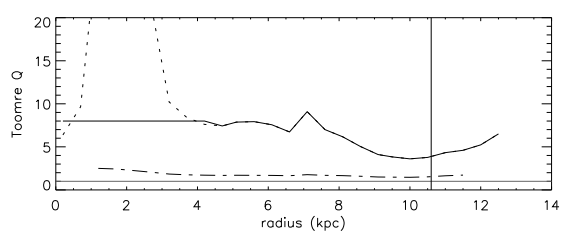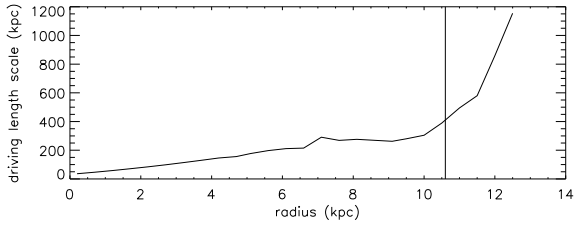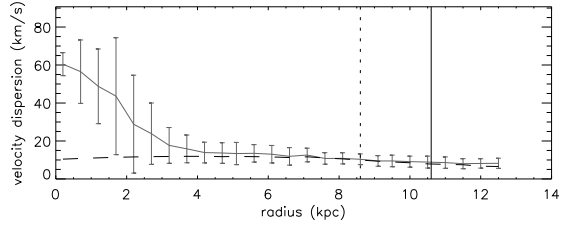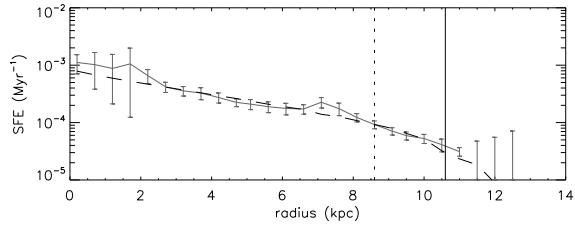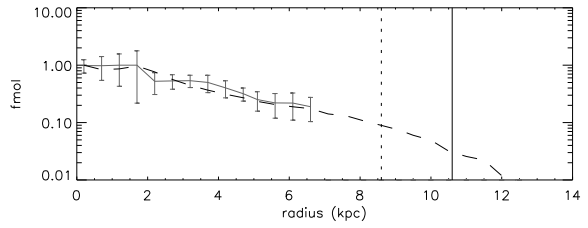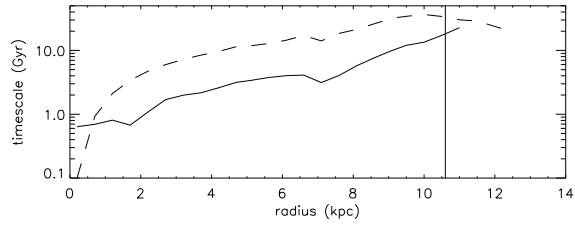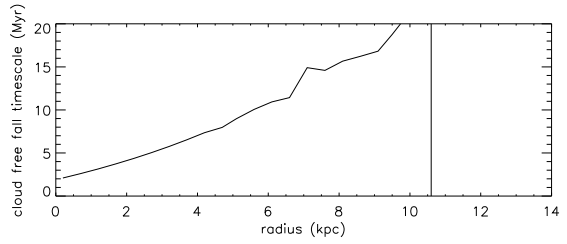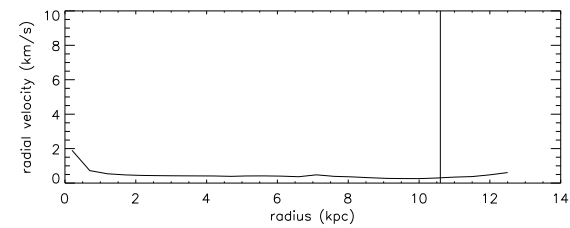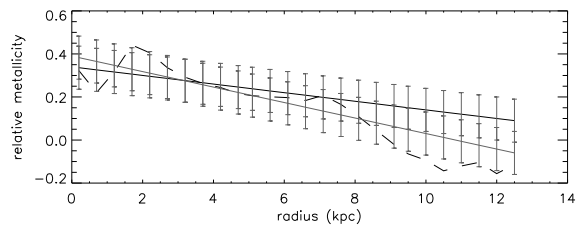

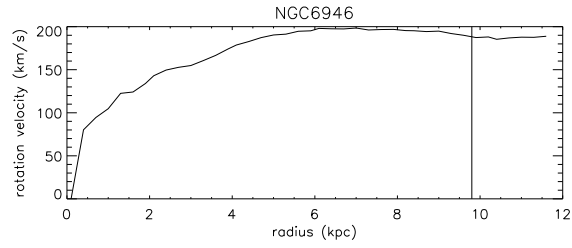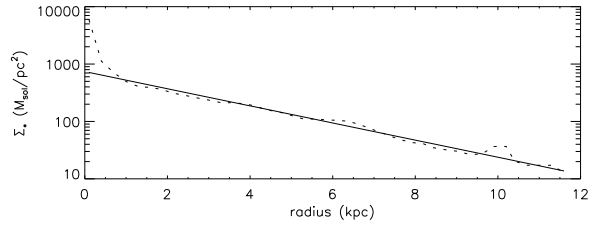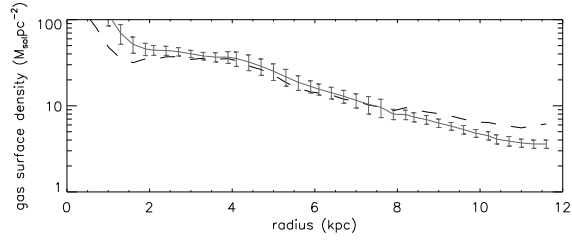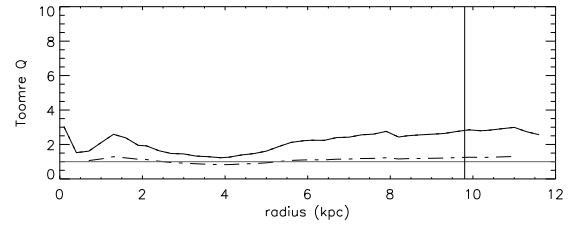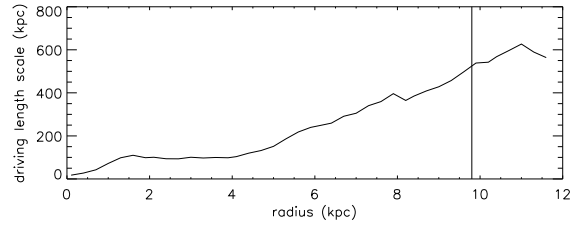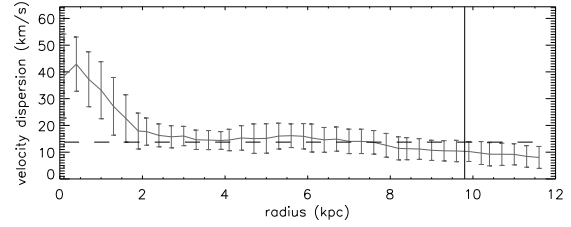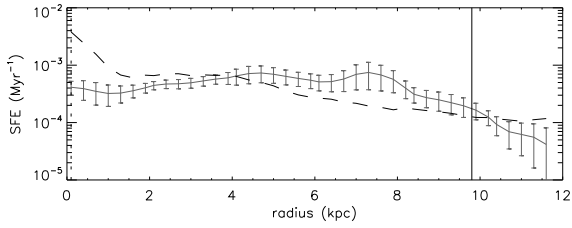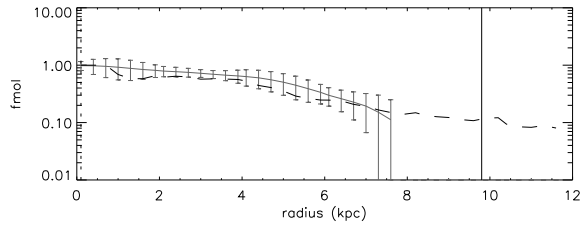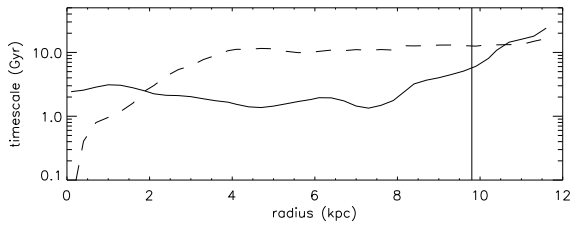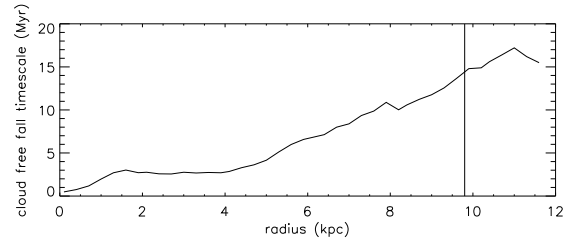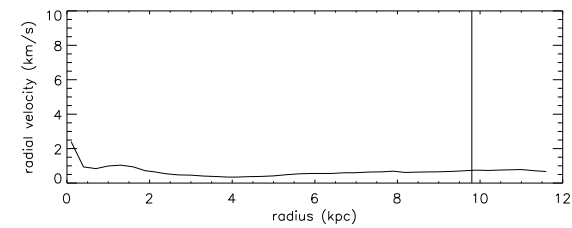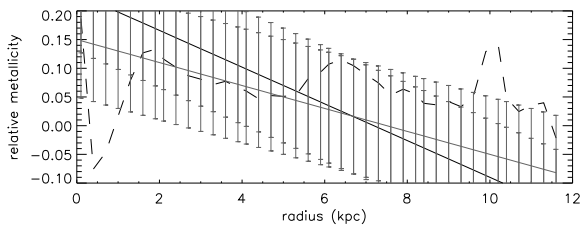

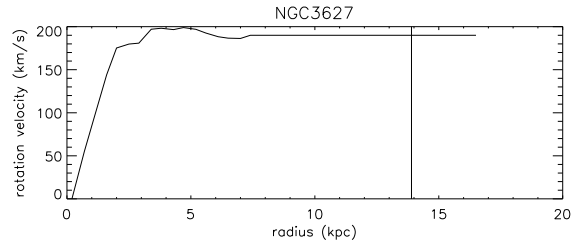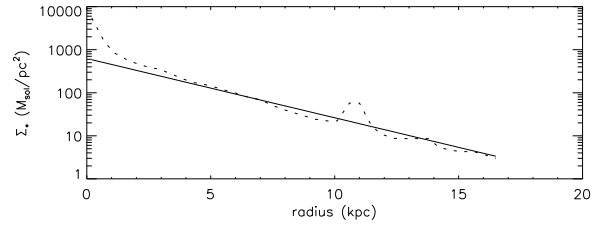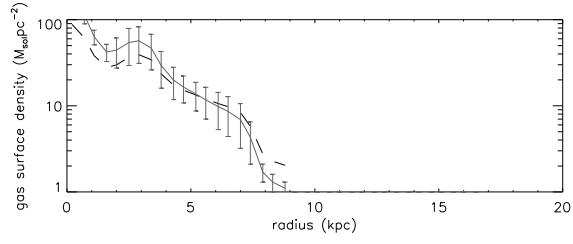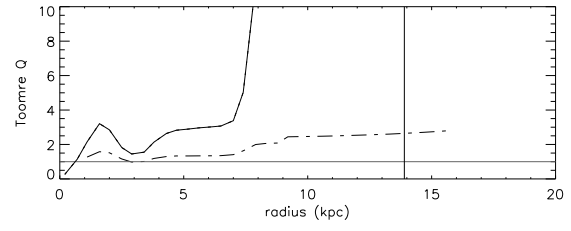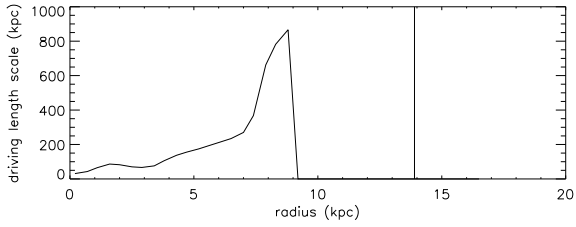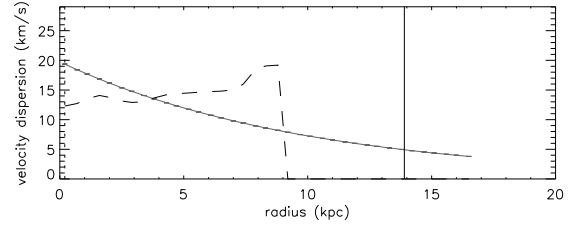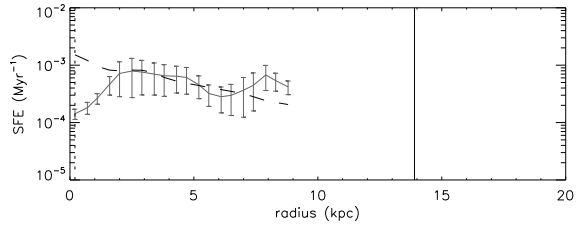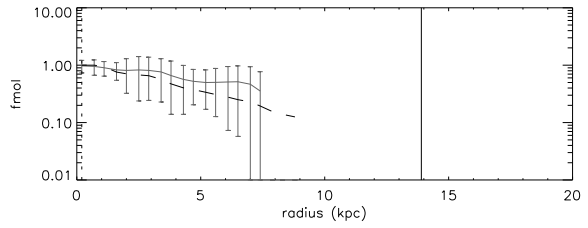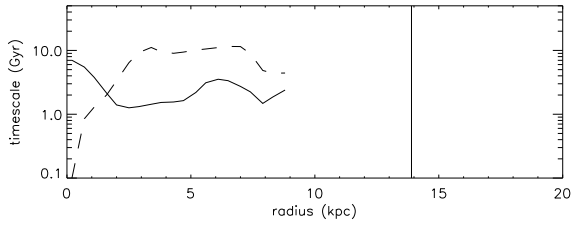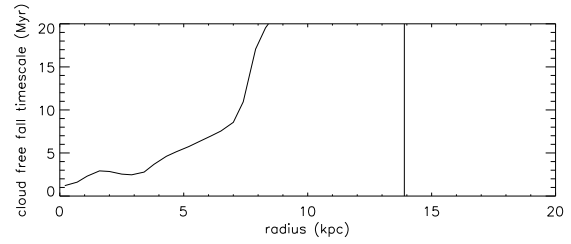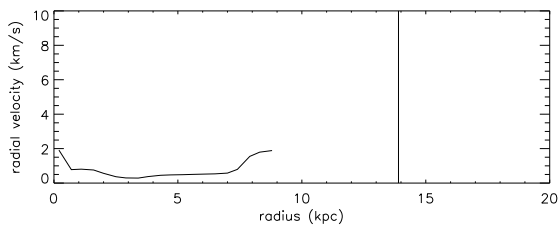

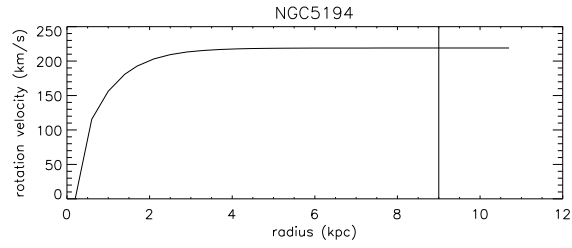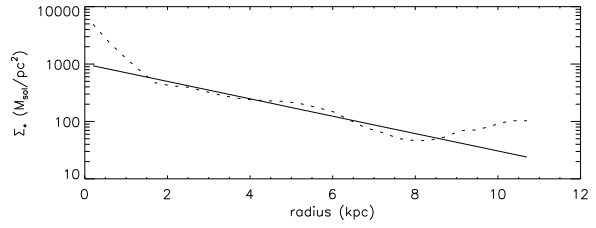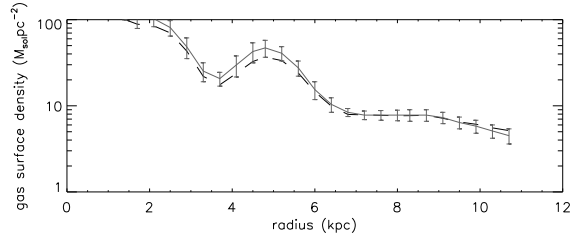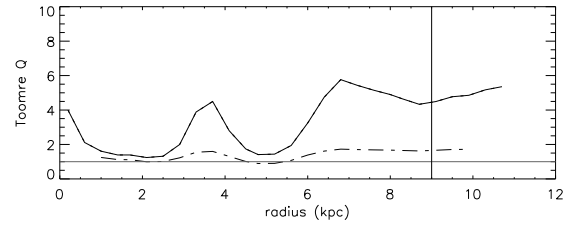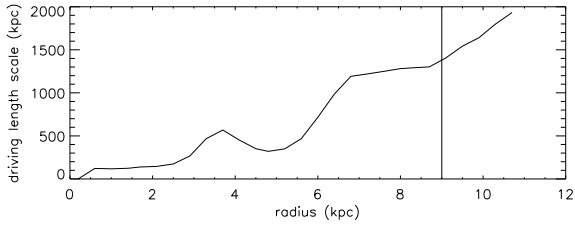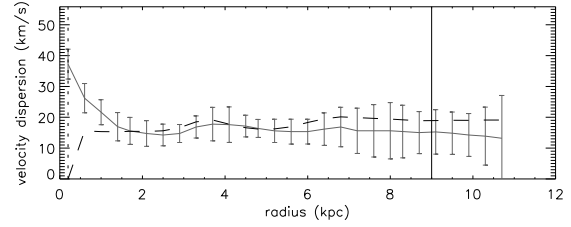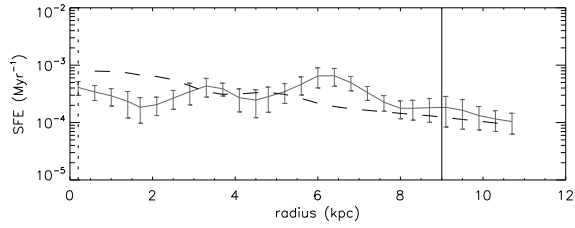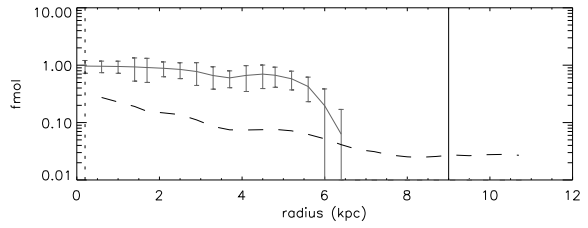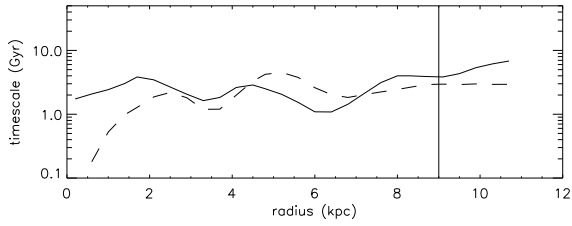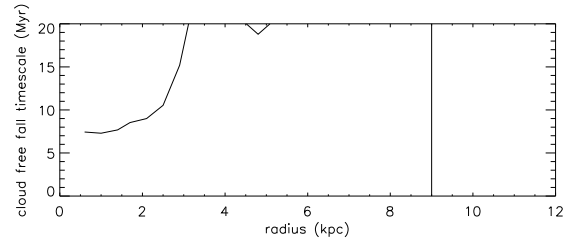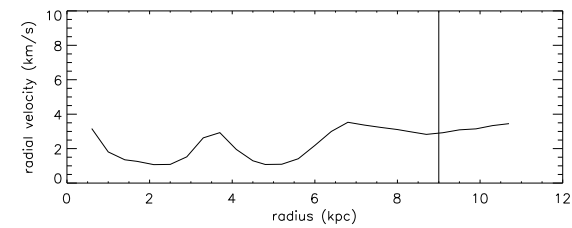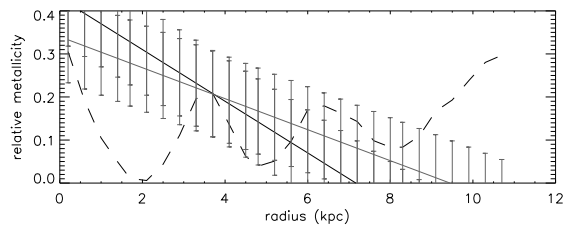

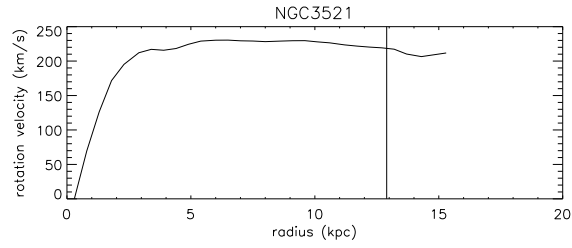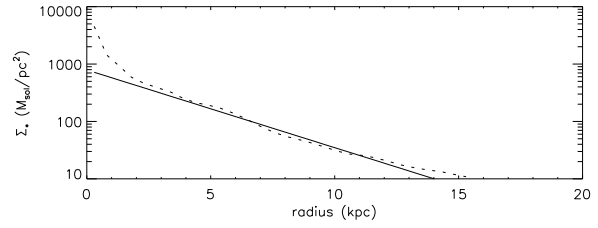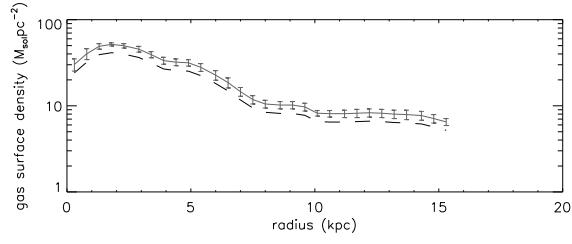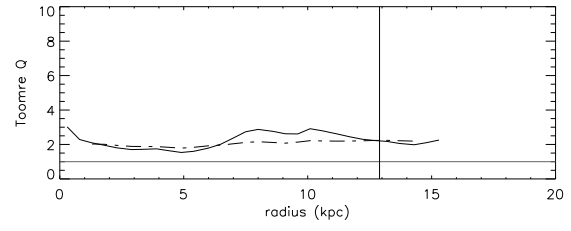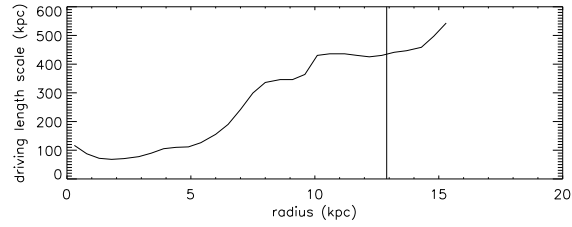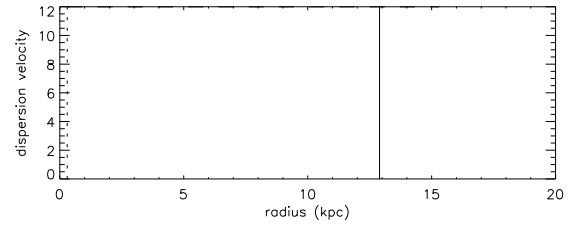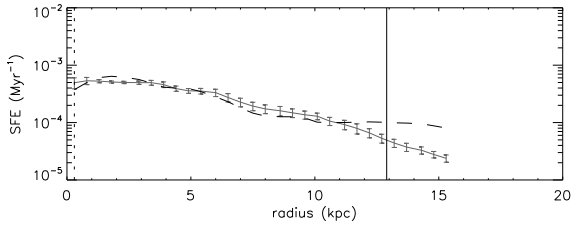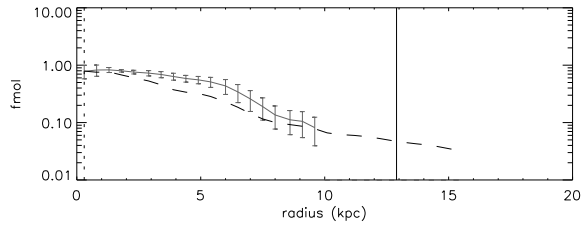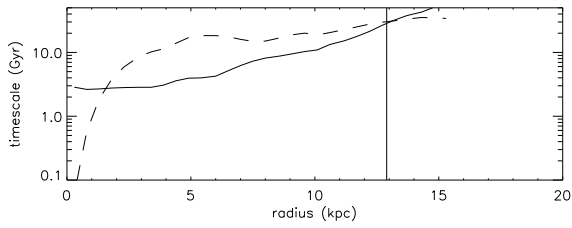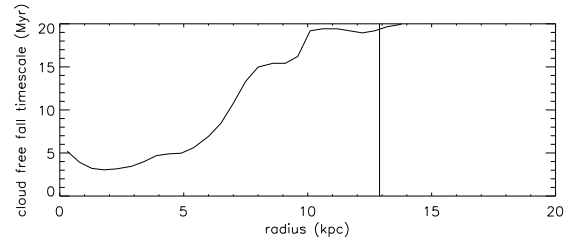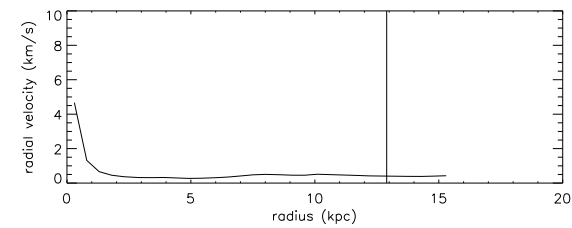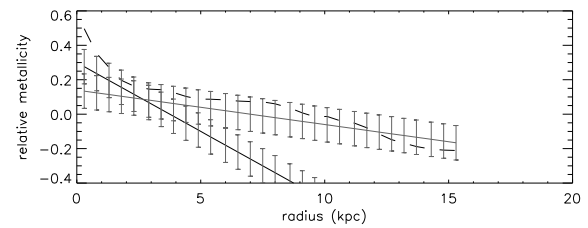

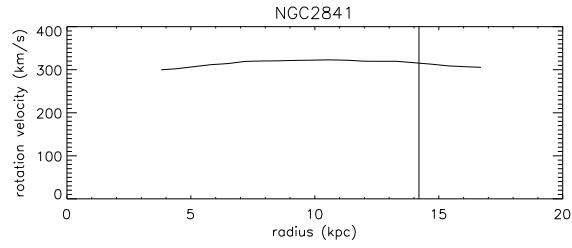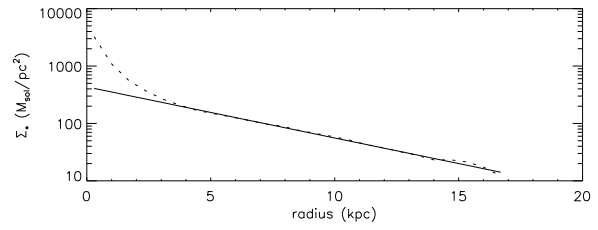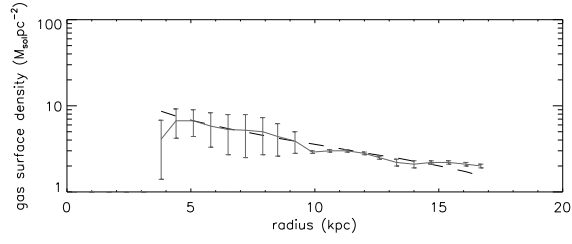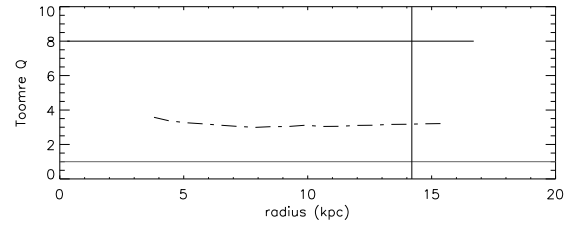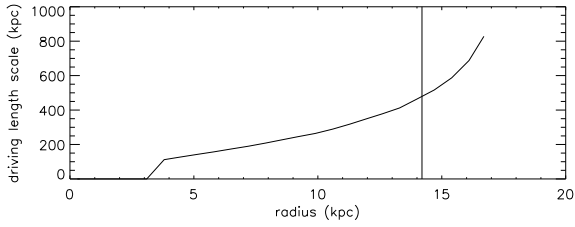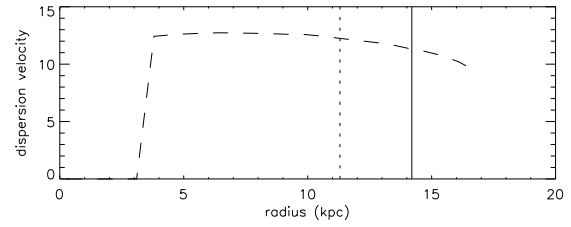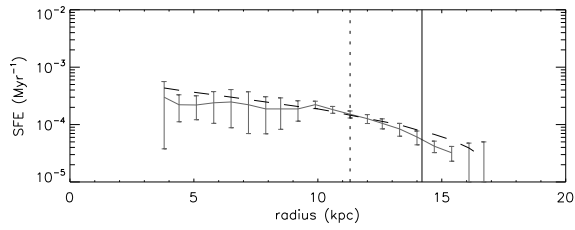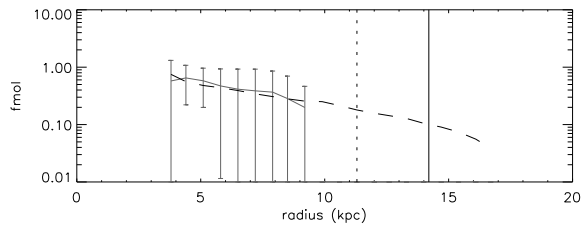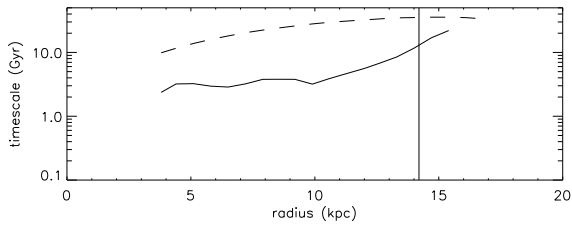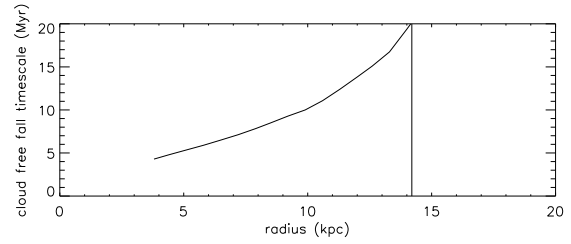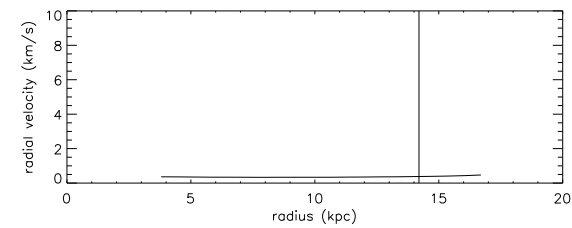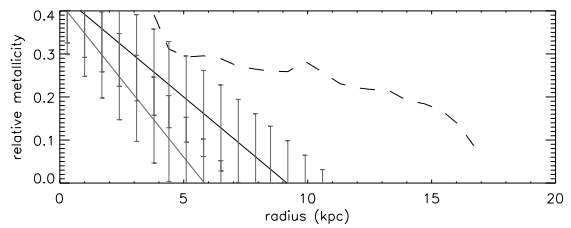



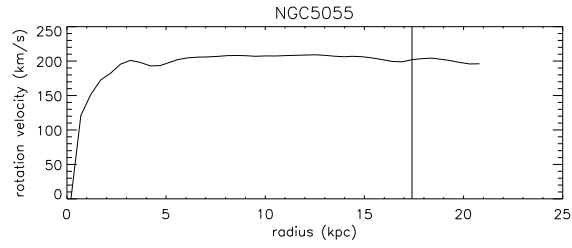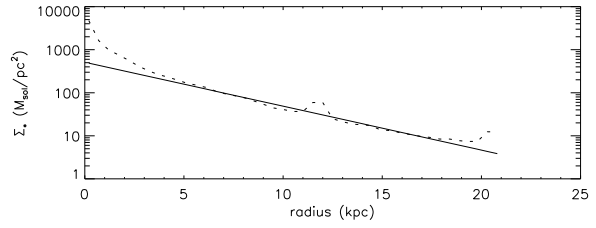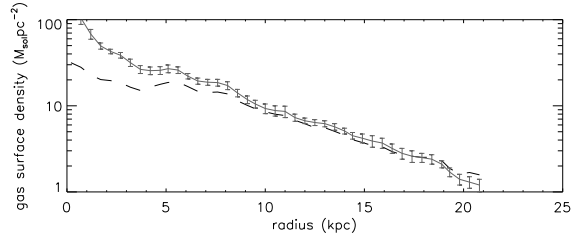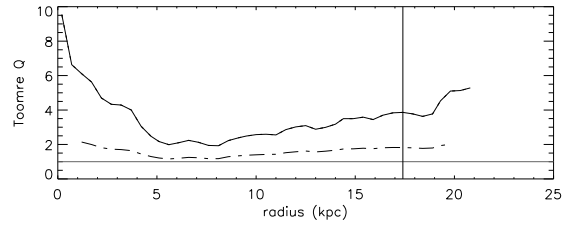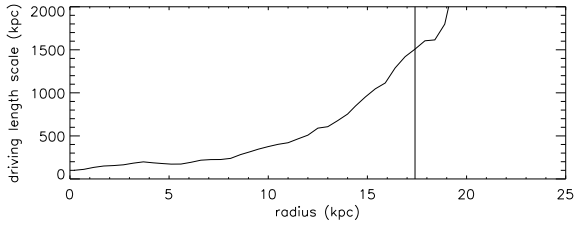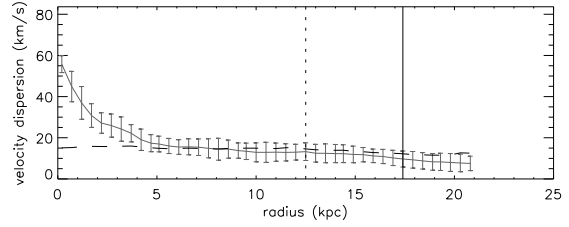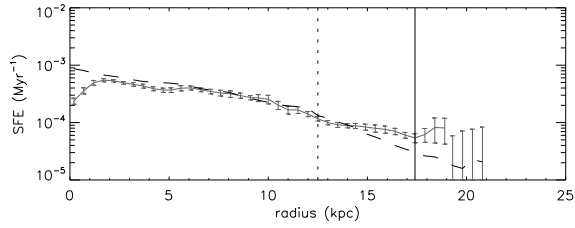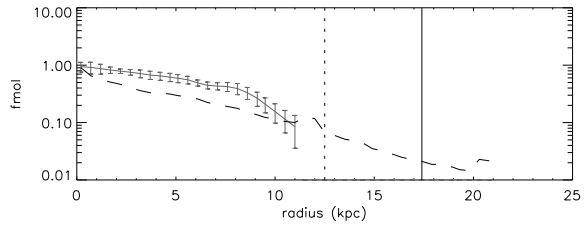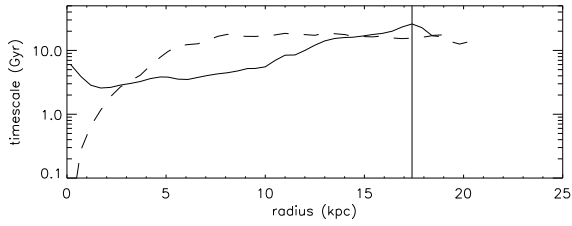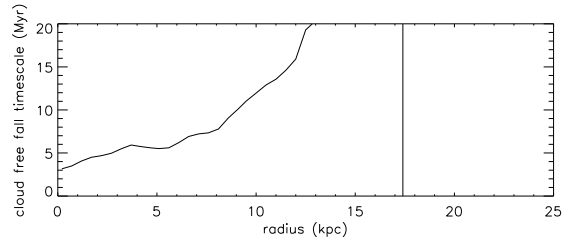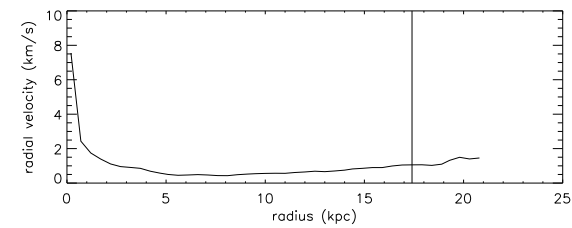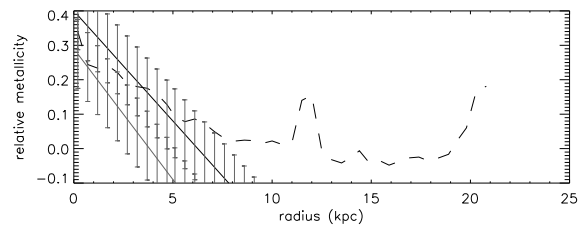

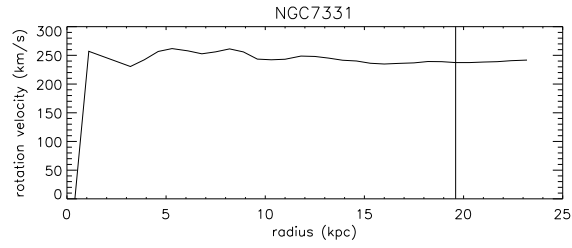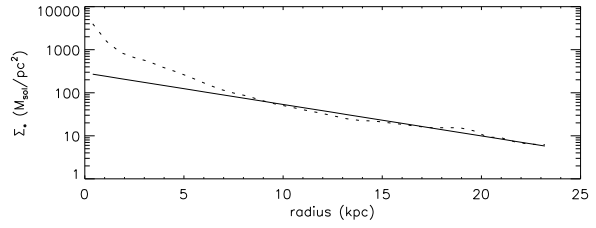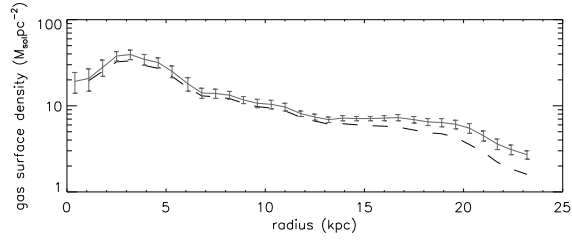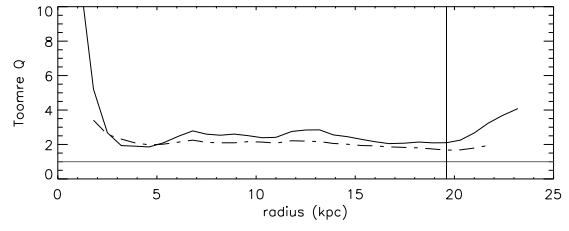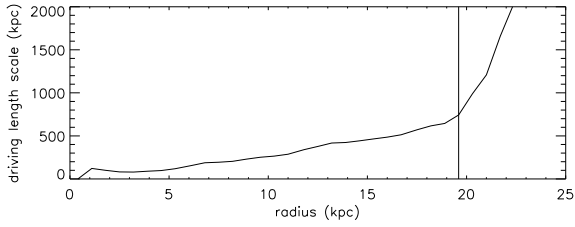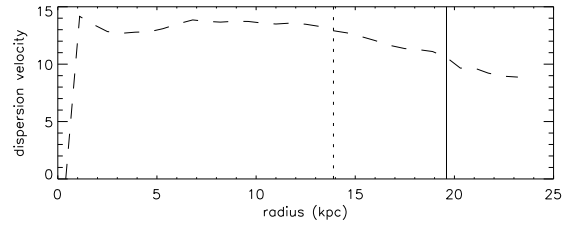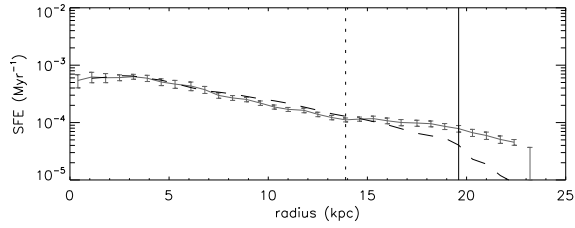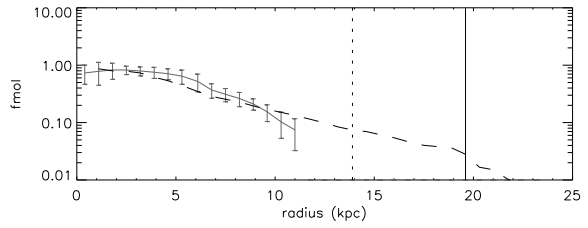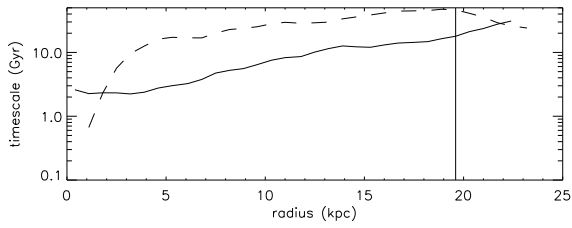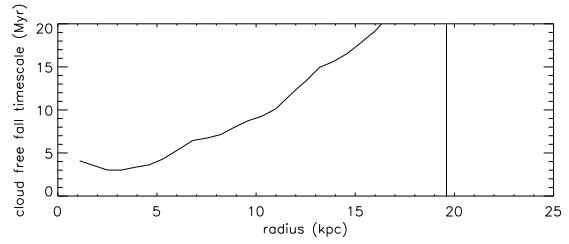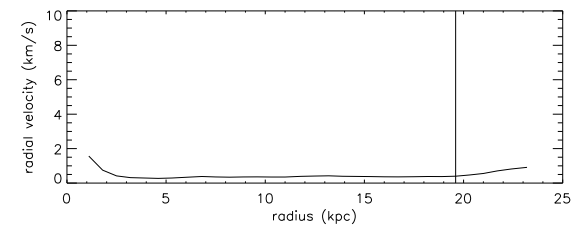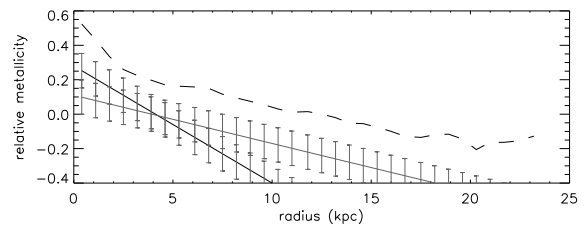

Supplement: Supplementary file 1 [file bvollmer_f1_full.pdf]
