# Supplementary material for: Sustaining star formation rates in spiral galaxies - Supernova-driven turbulent accretion disk models applied to THINGS galaxies
Source: arXiv:1009.3722 ancillary file (2010-09-20)

IC2574

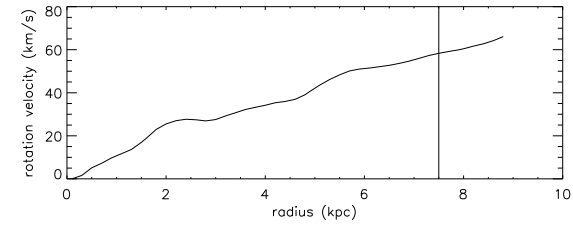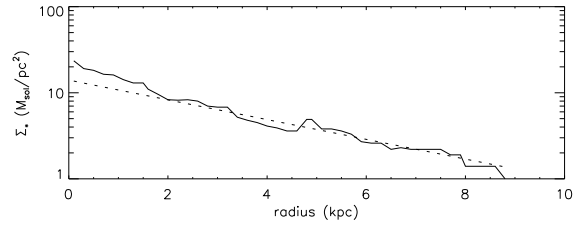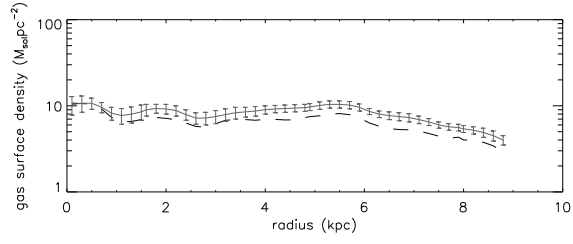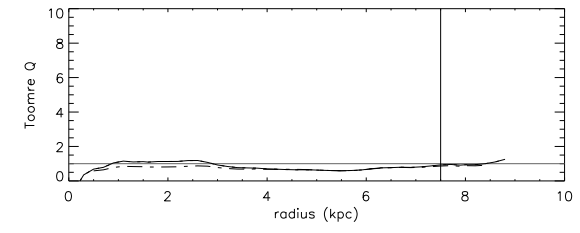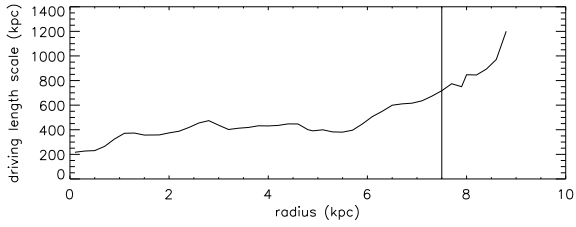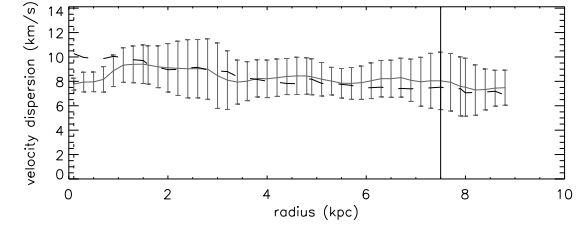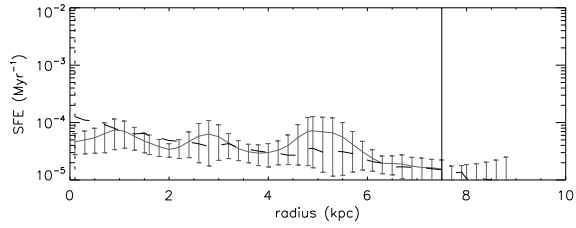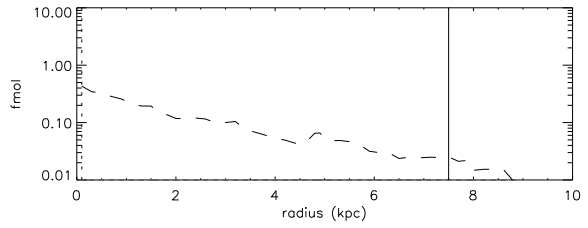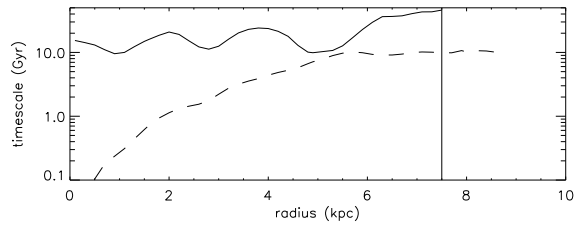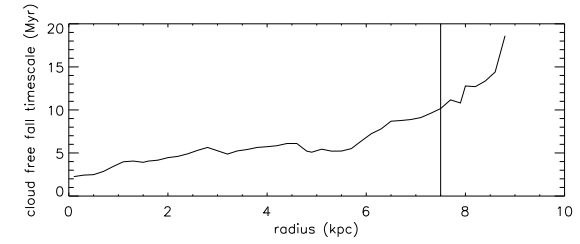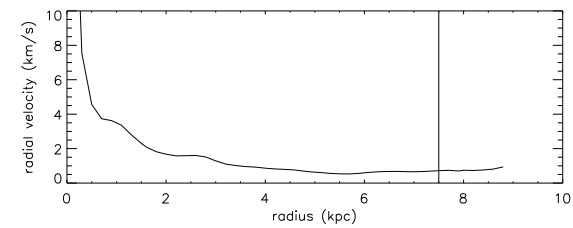

NGC4214

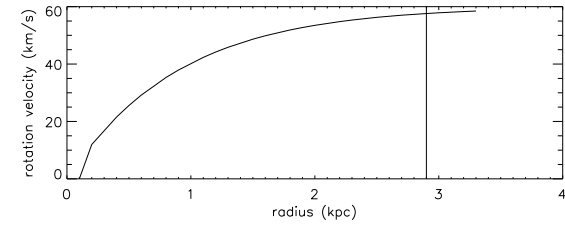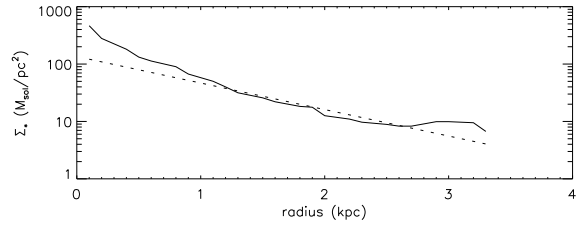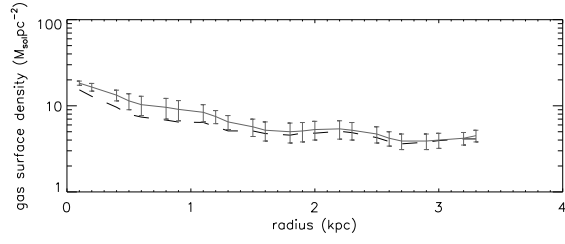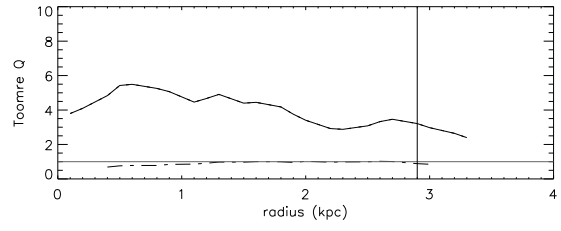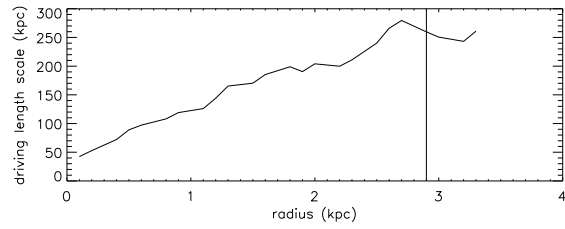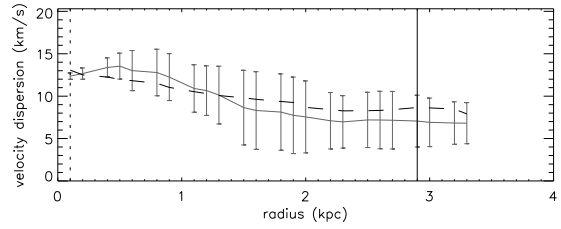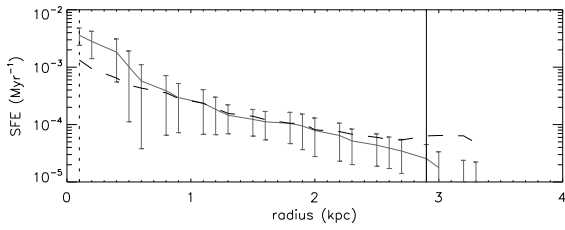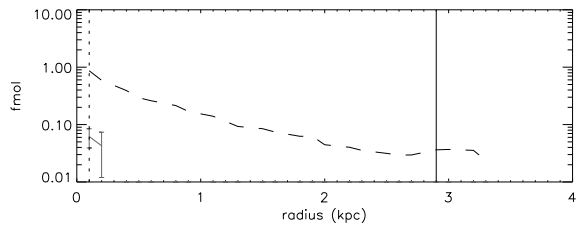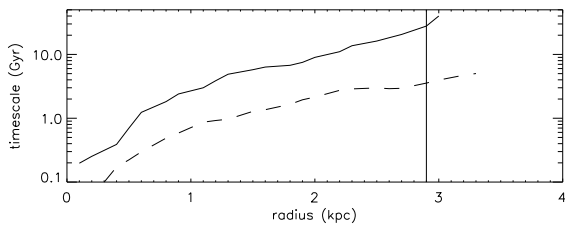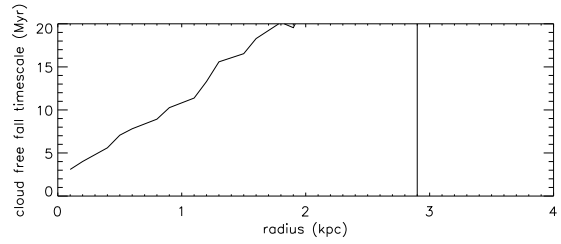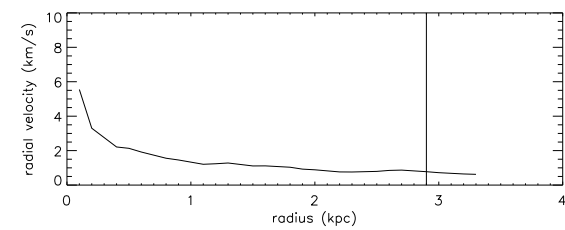

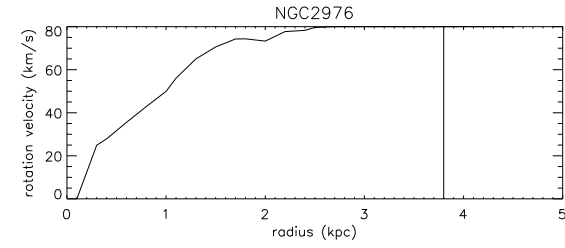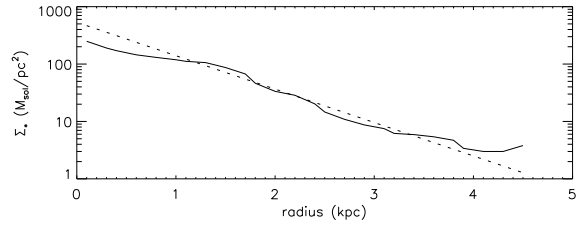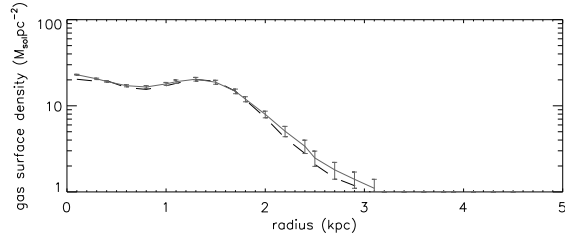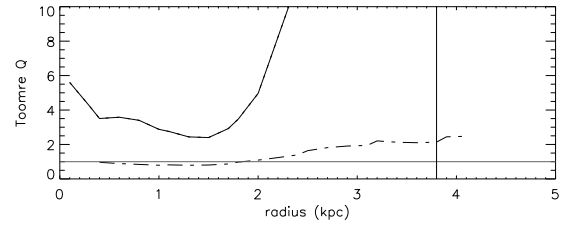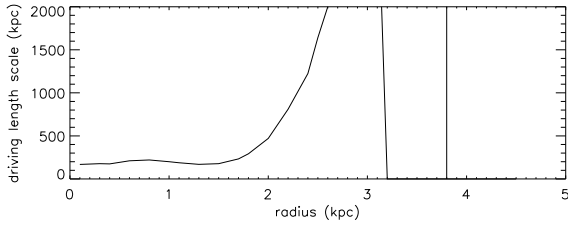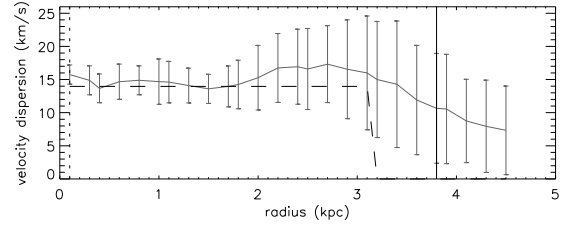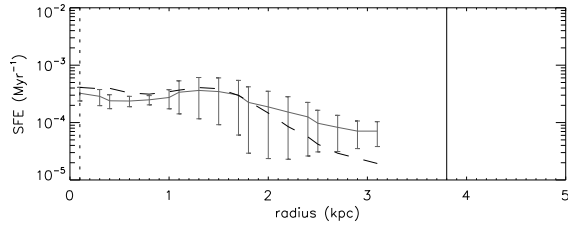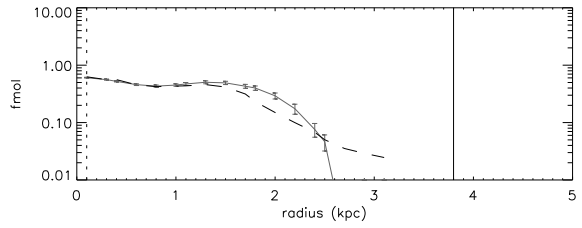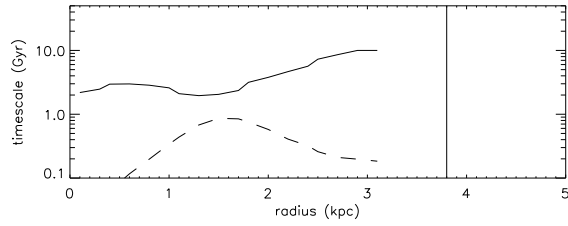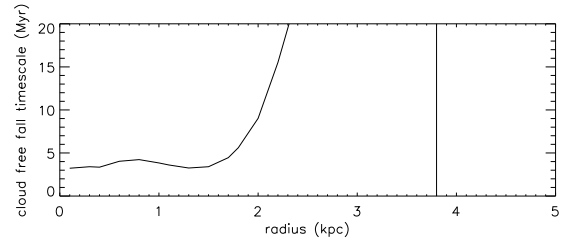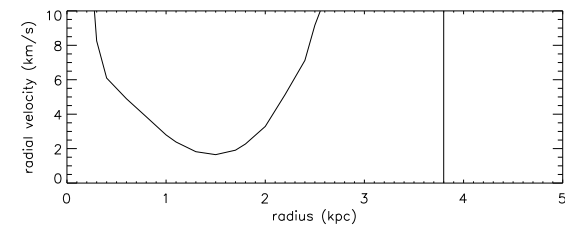

NGC7793

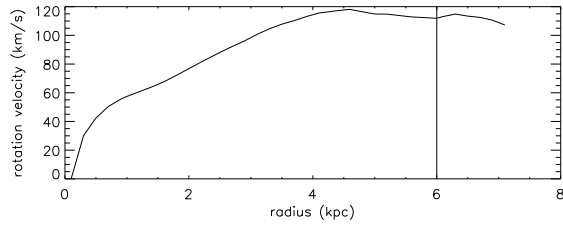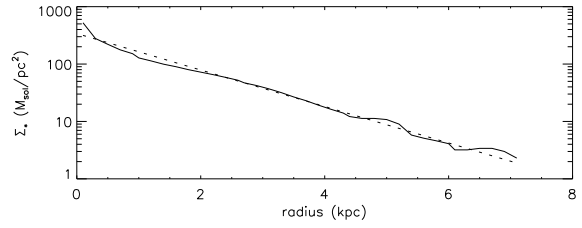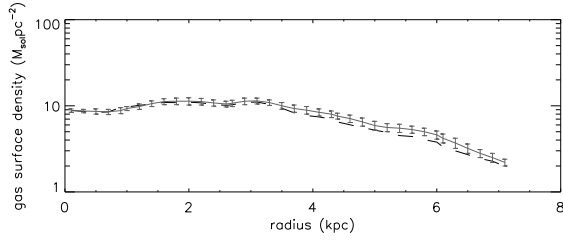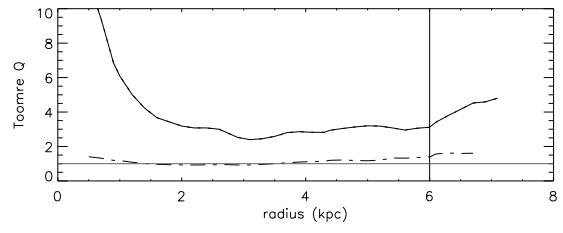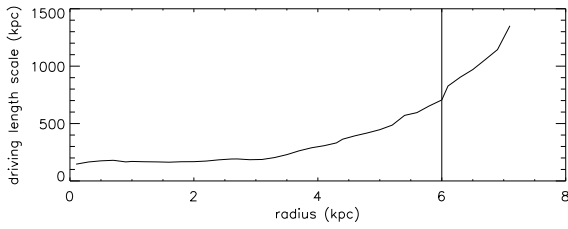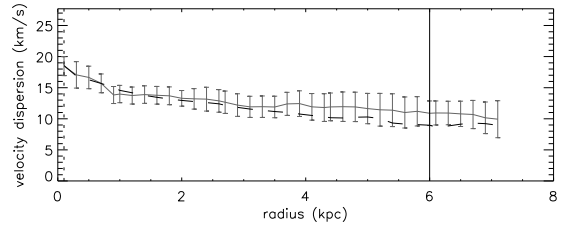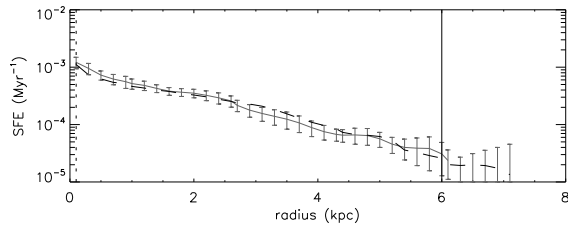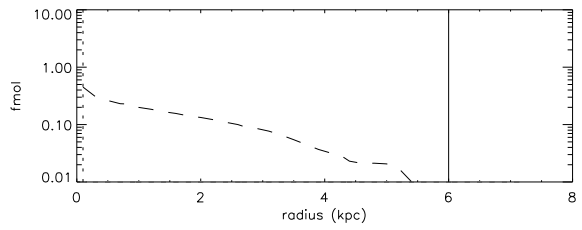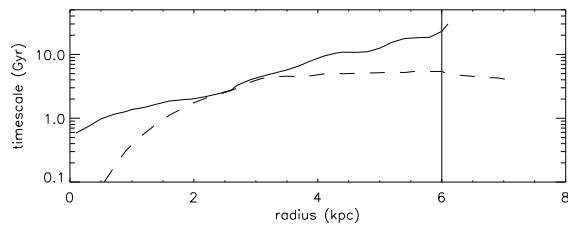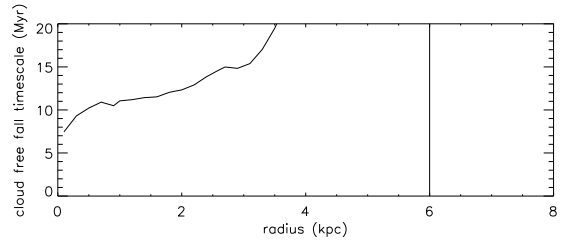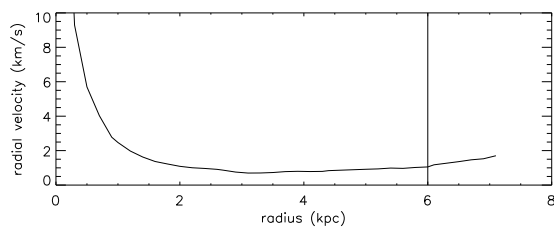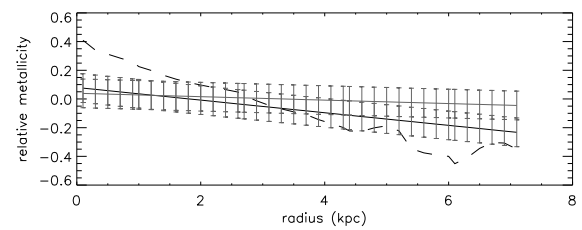

NGC2403

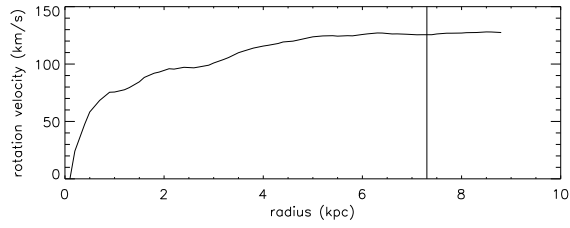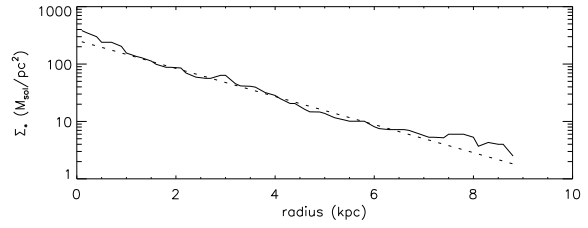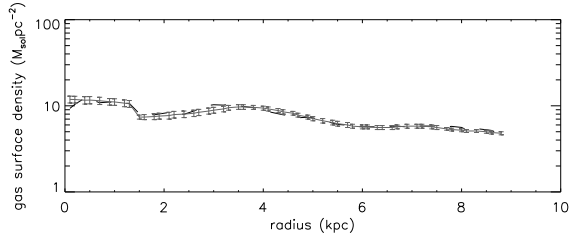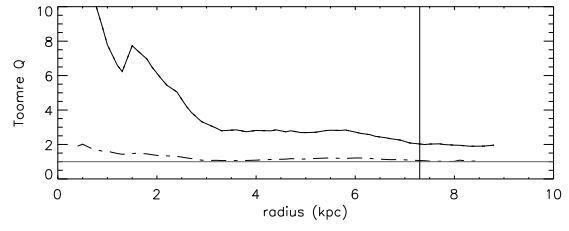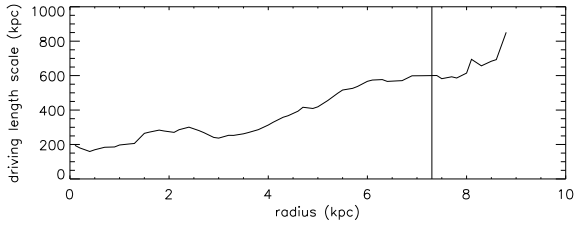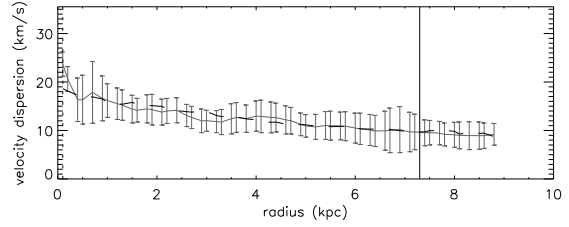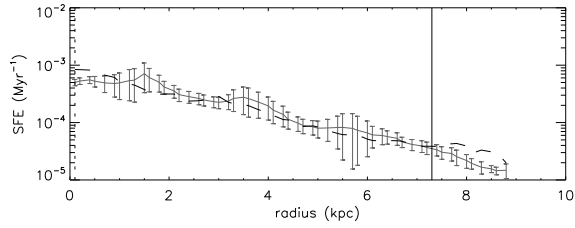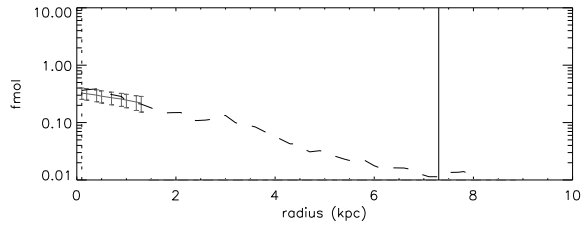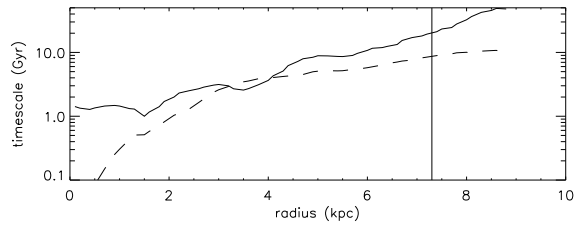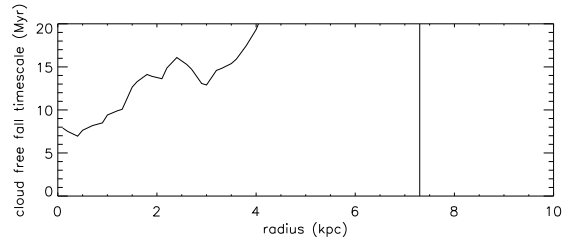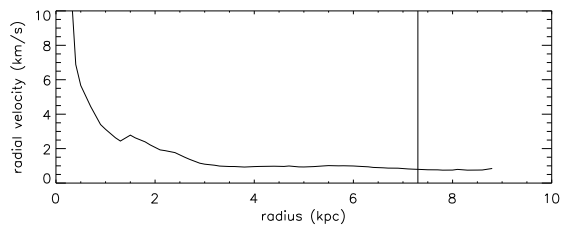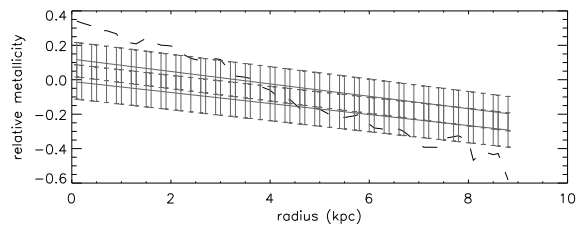

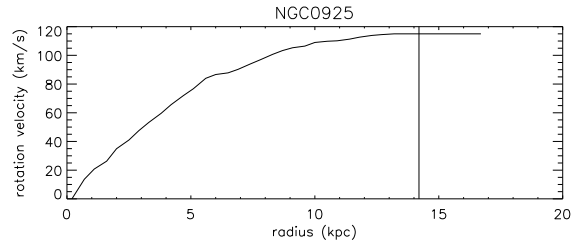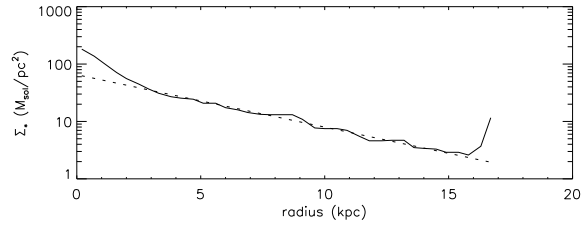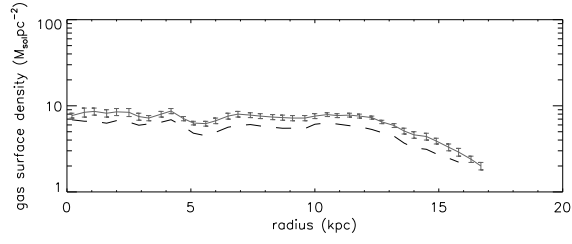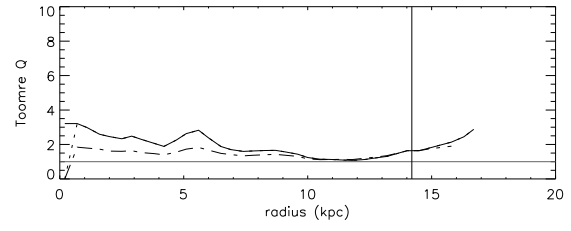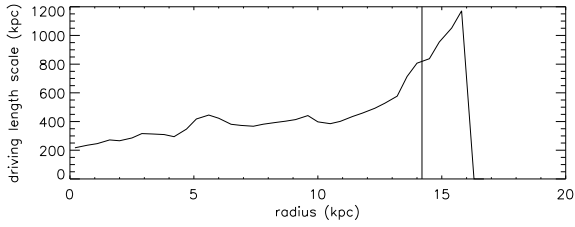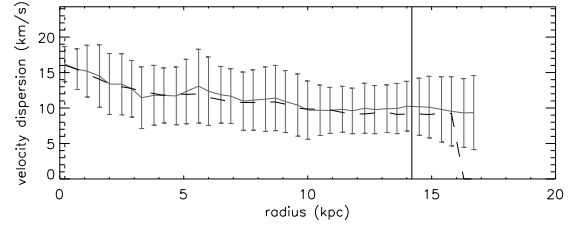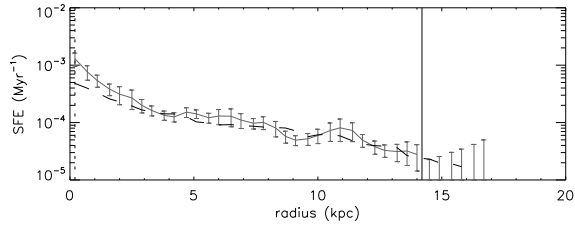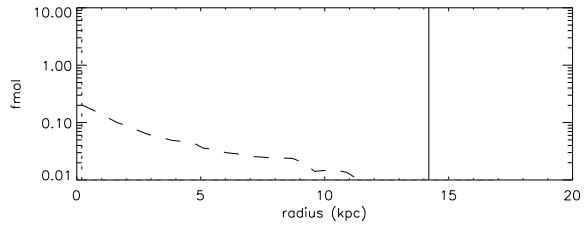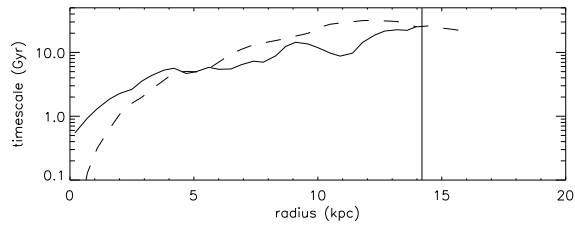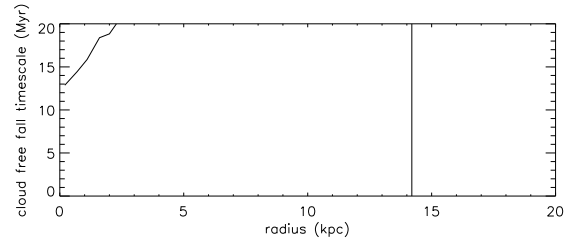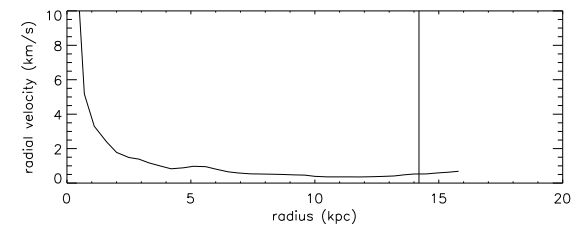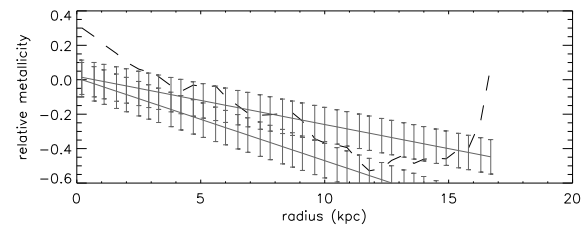

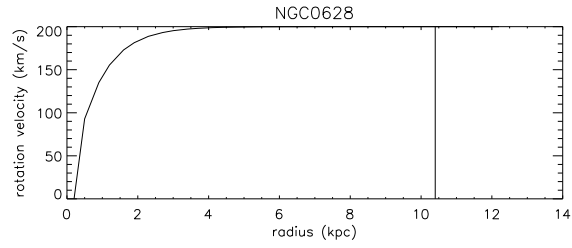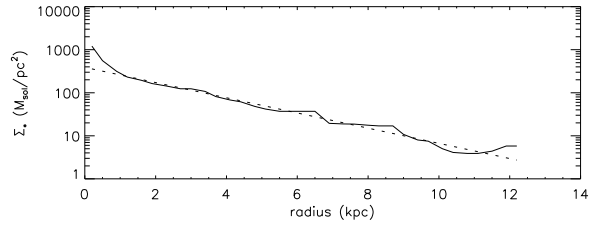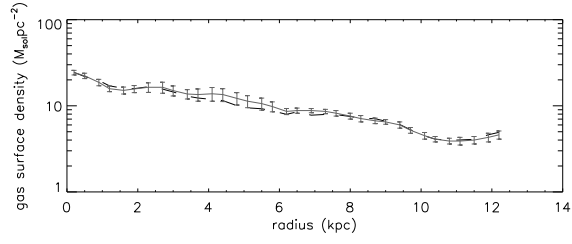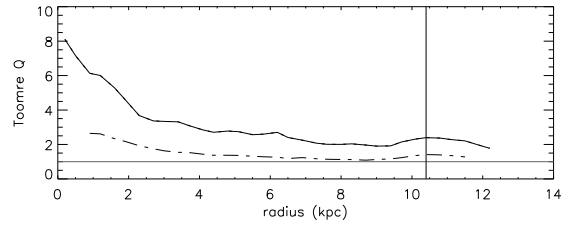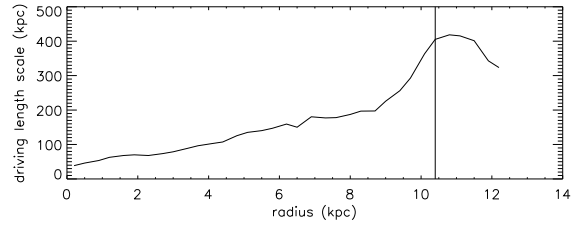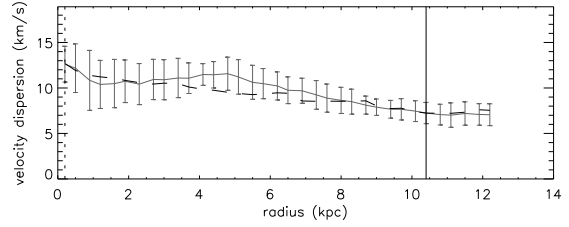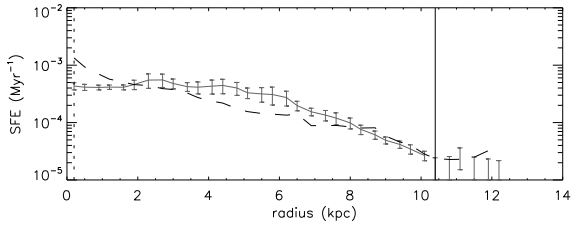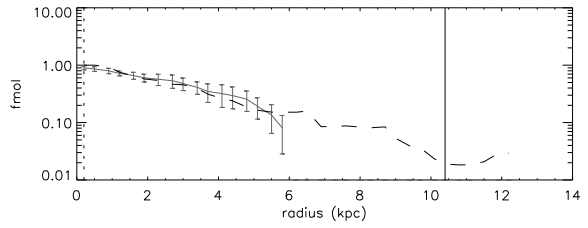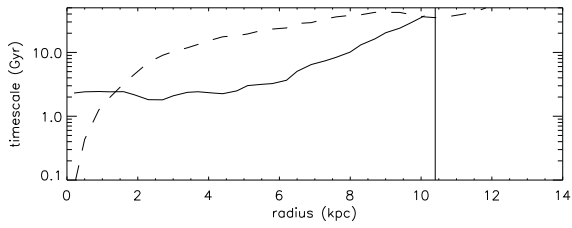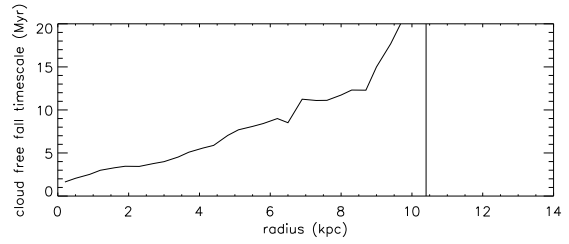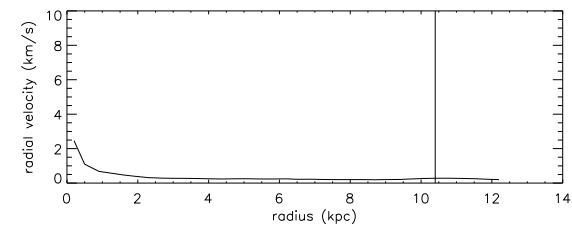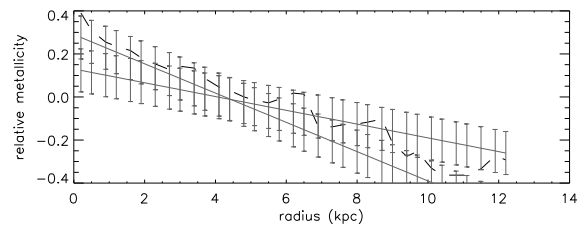

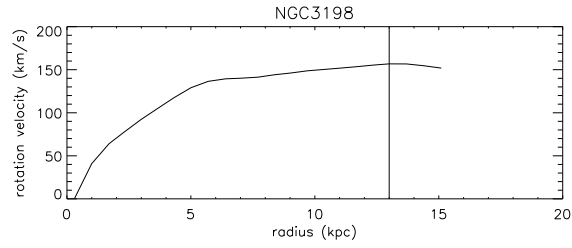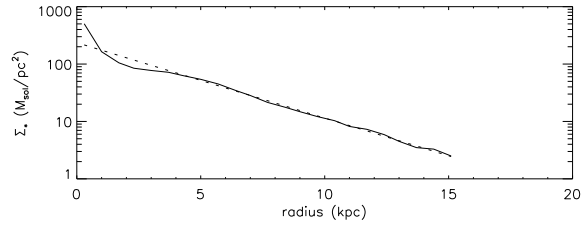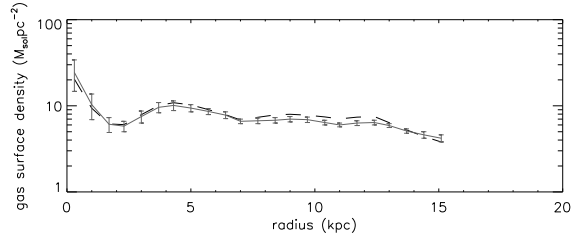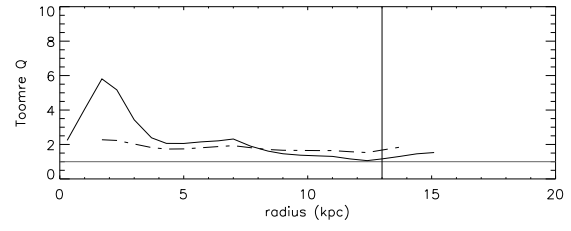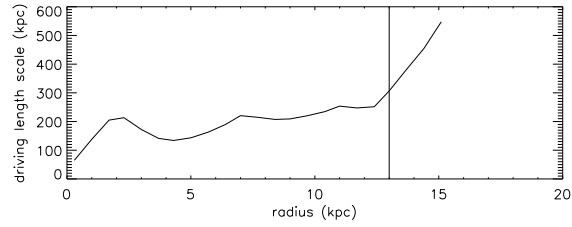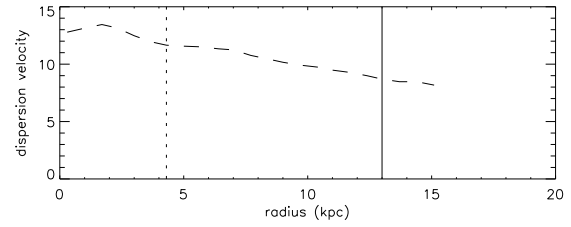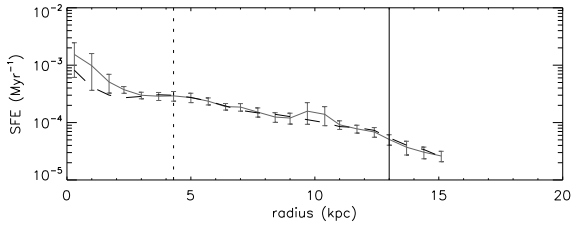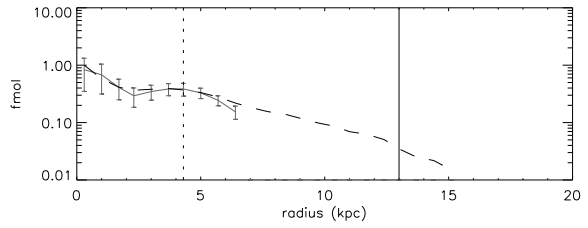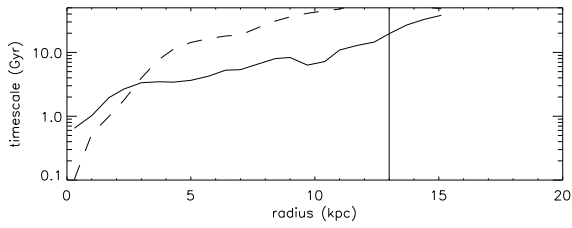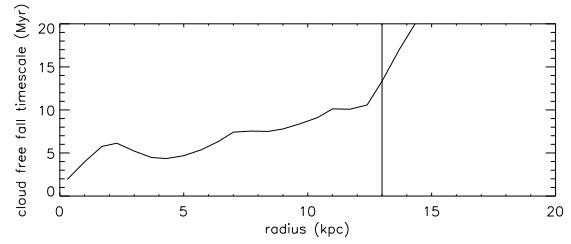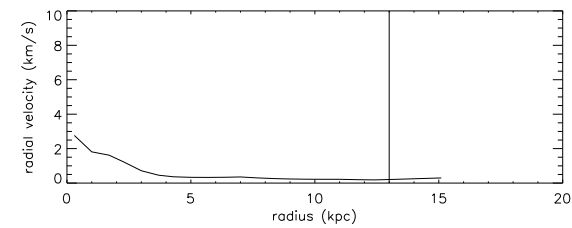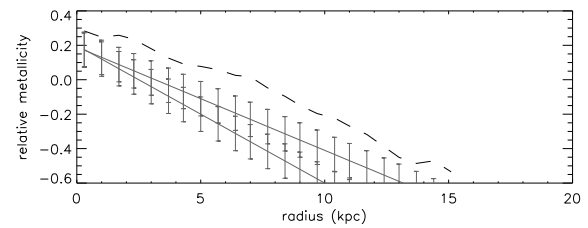



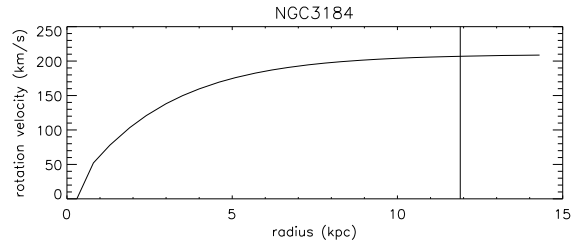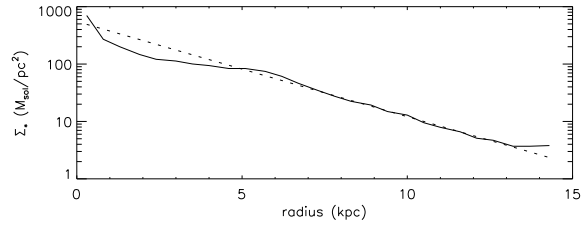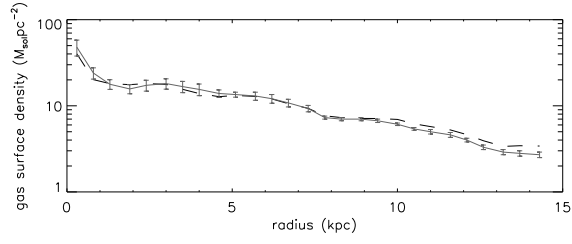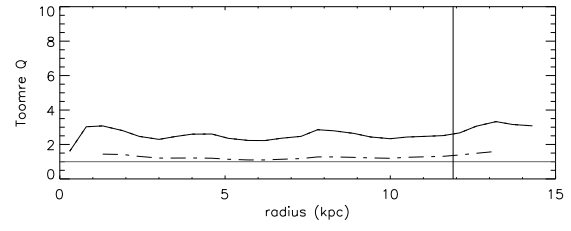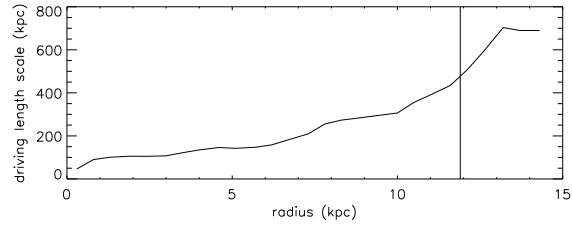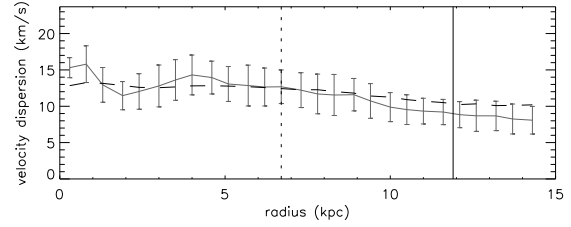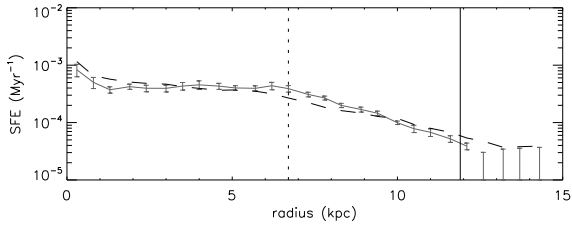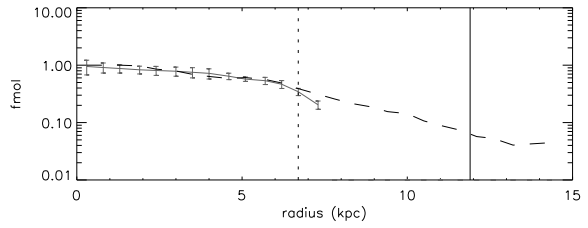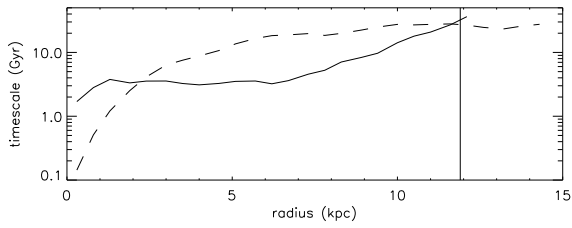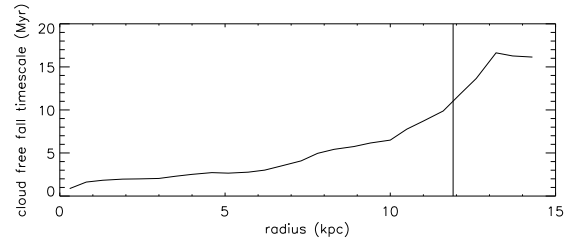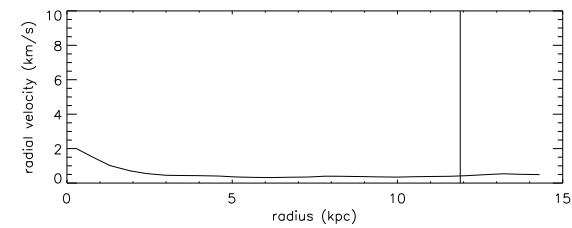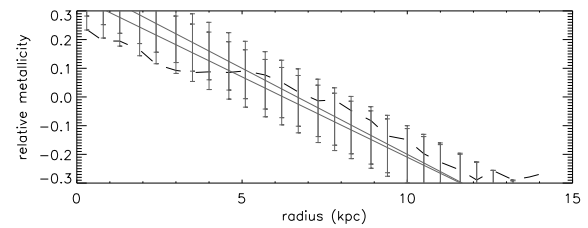

NGC4736

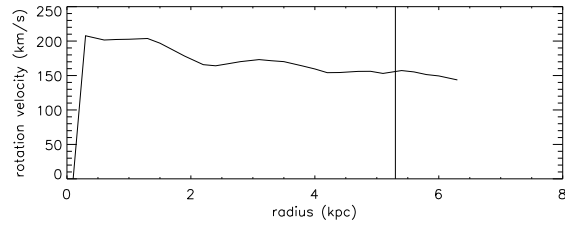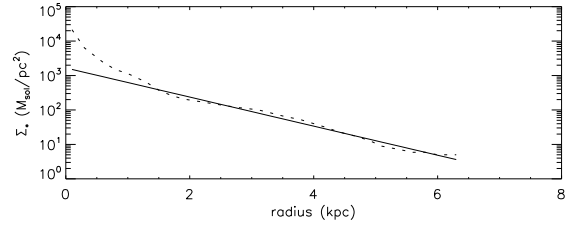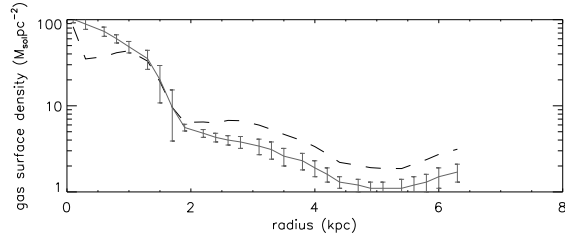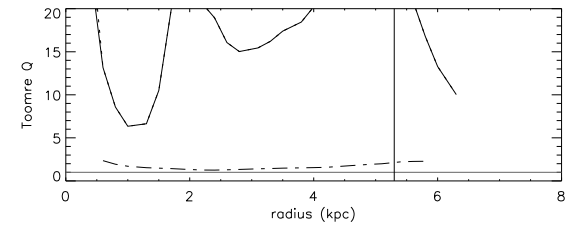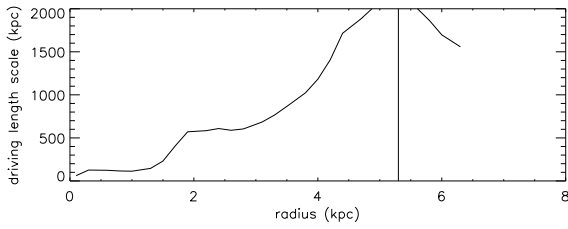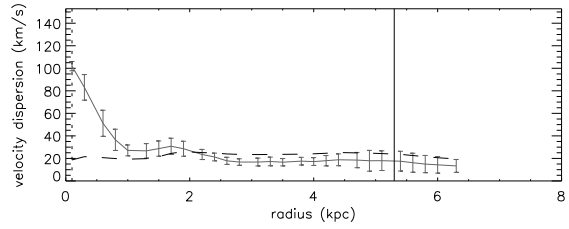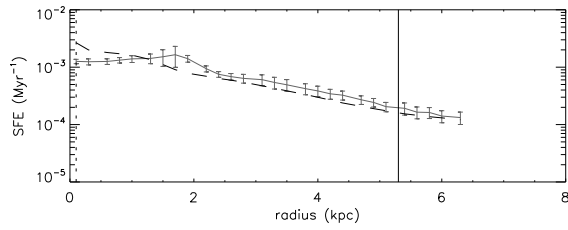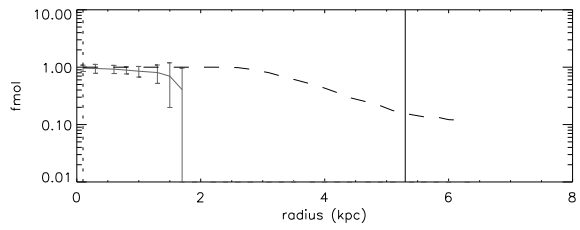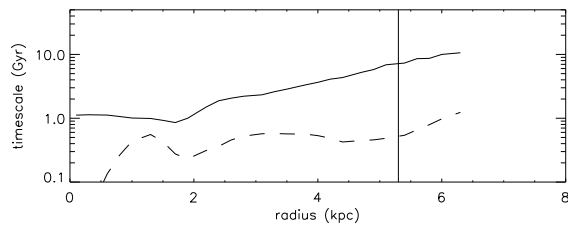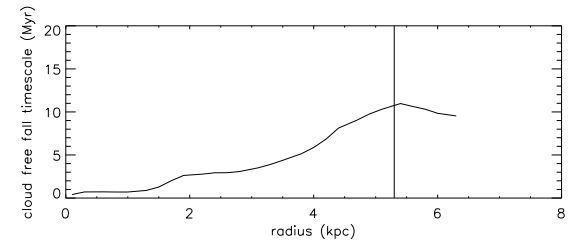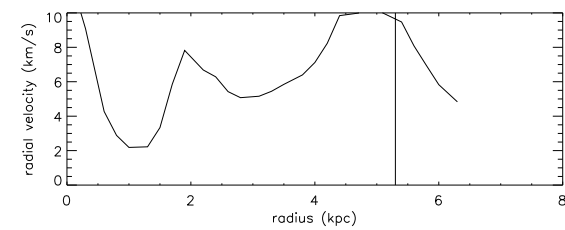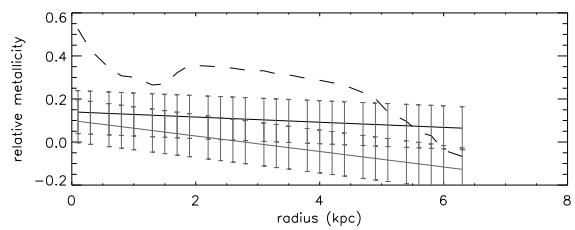

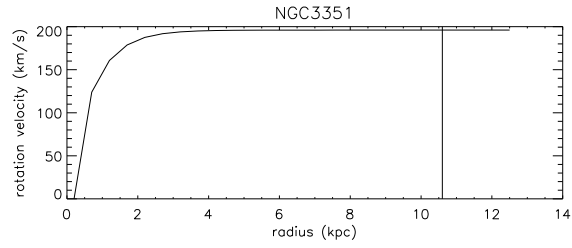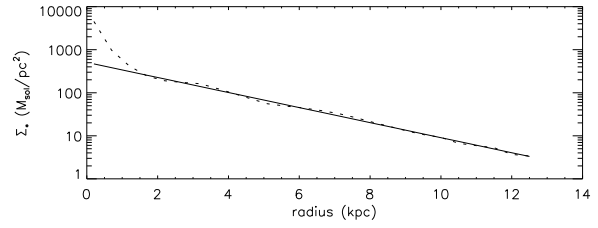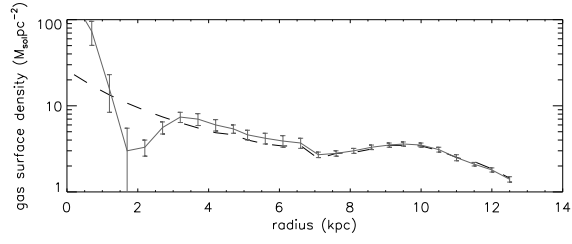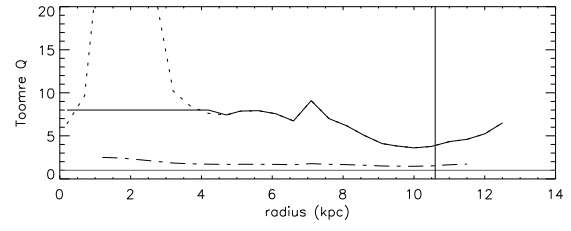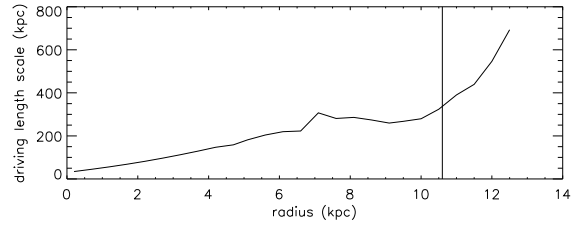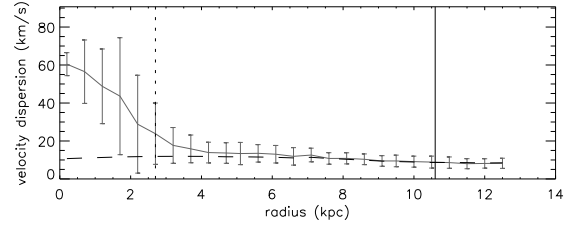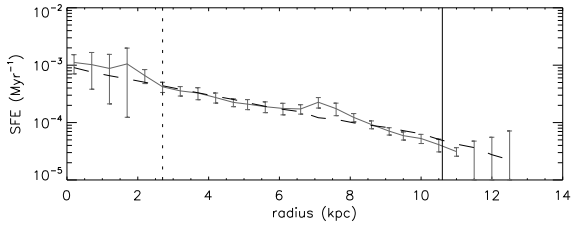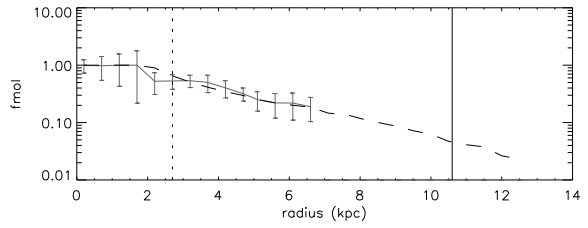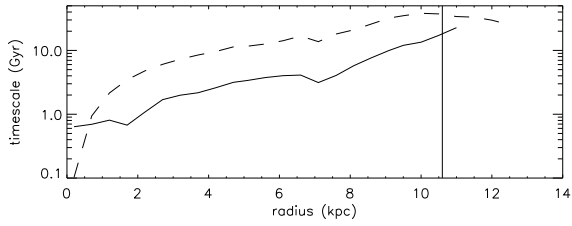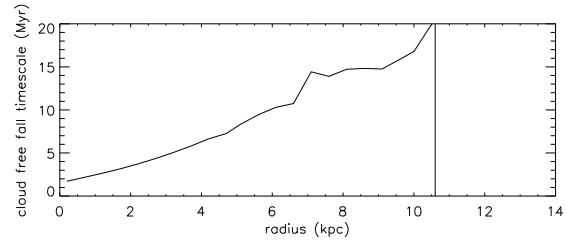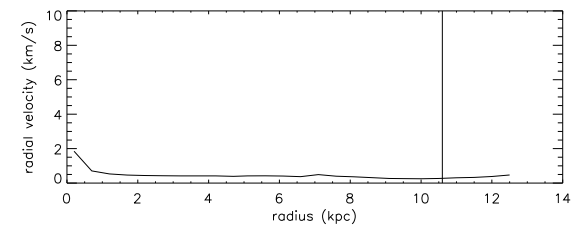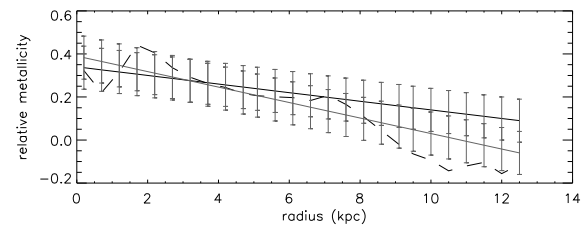

NGC6946

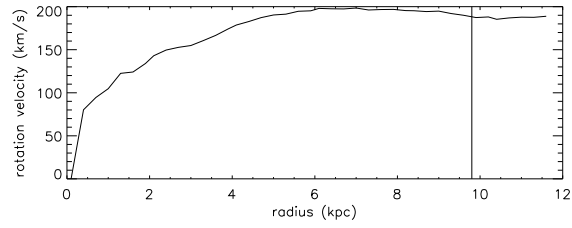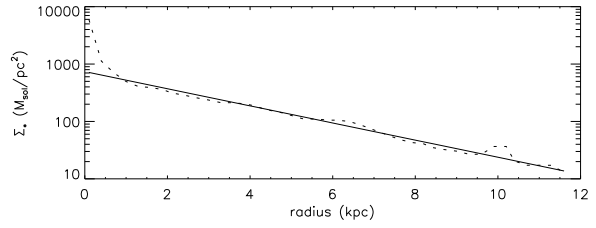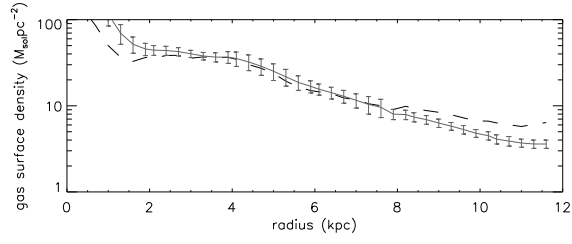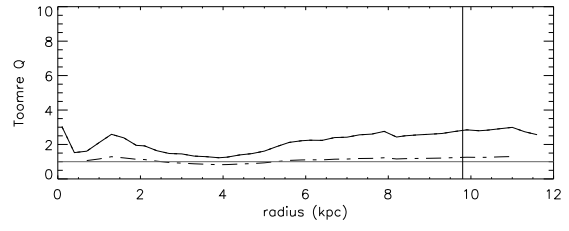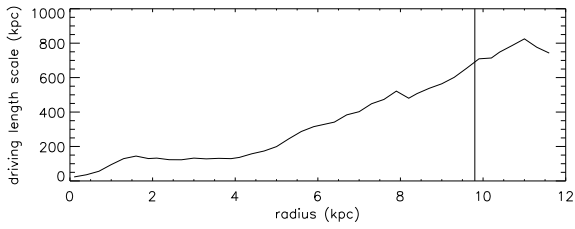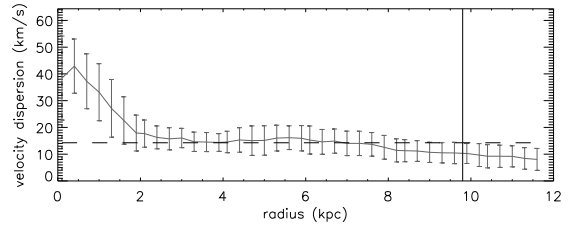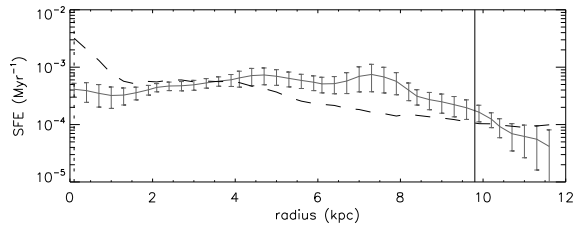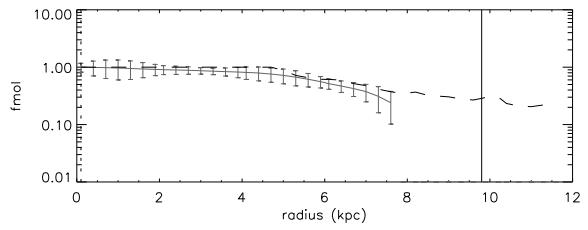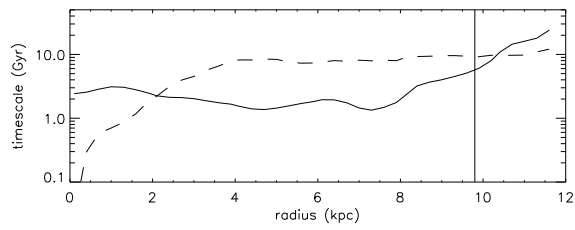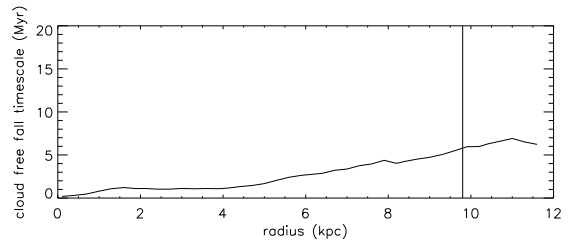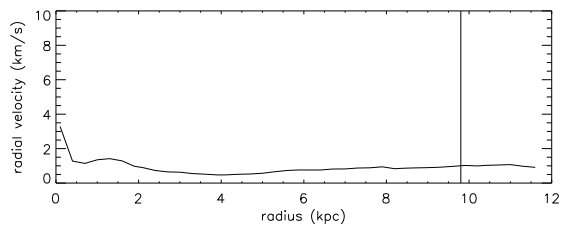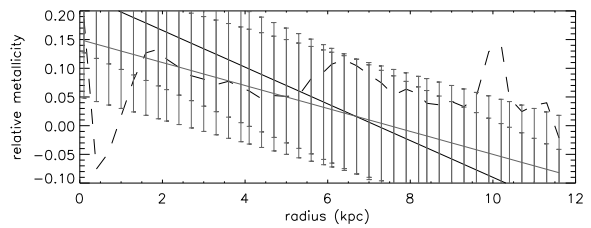

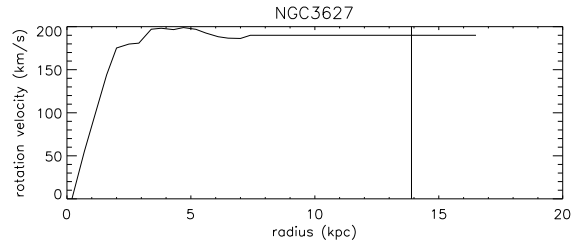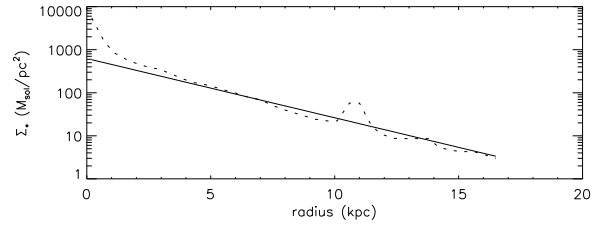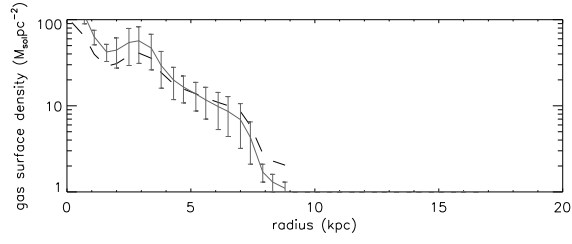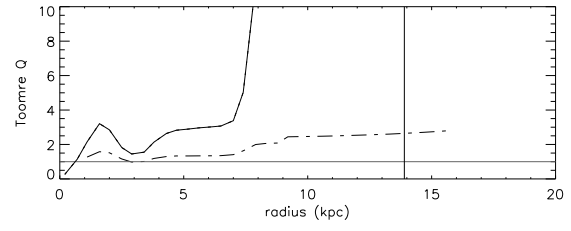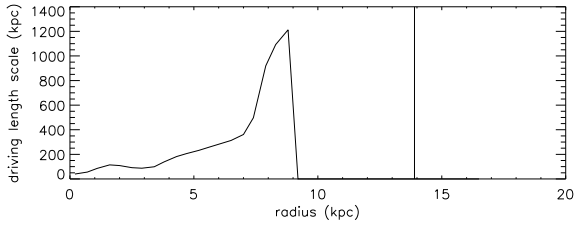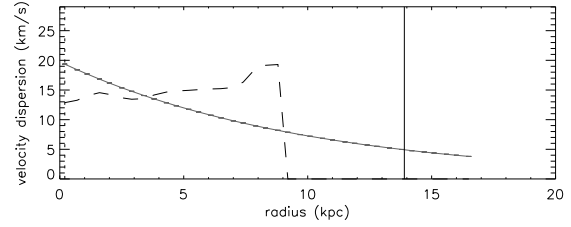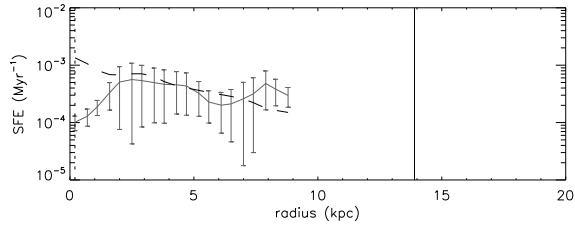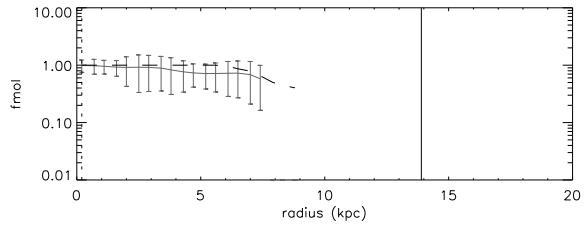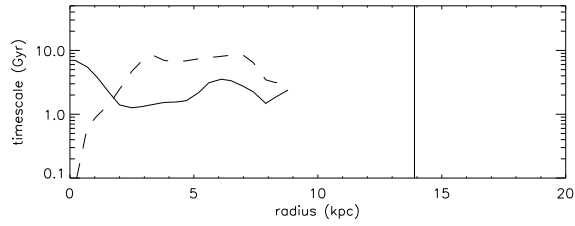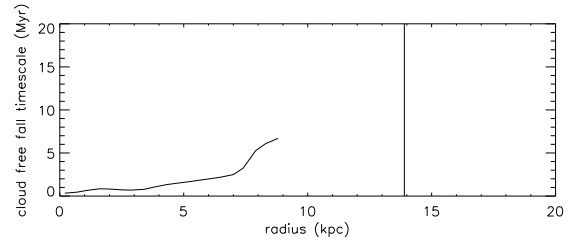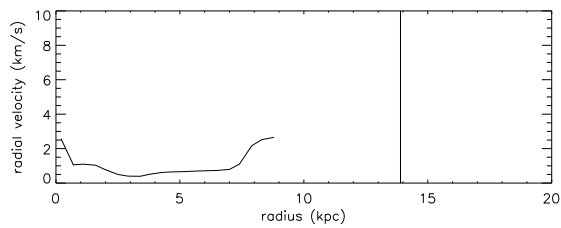

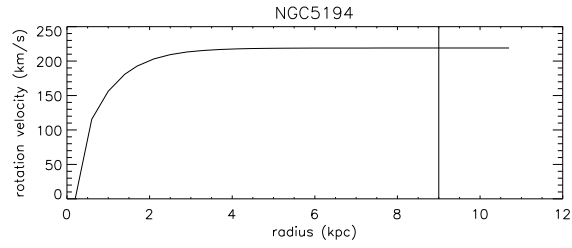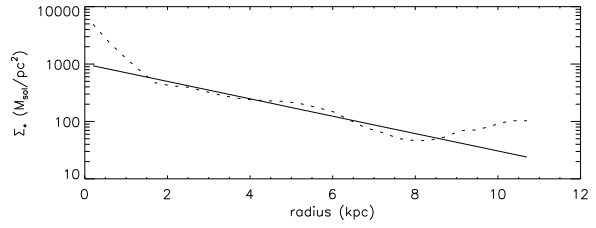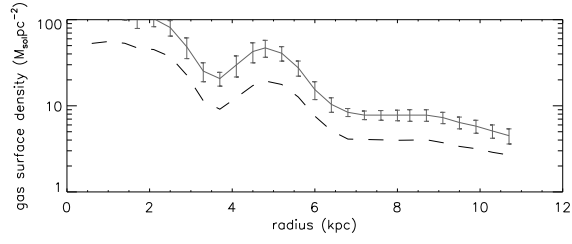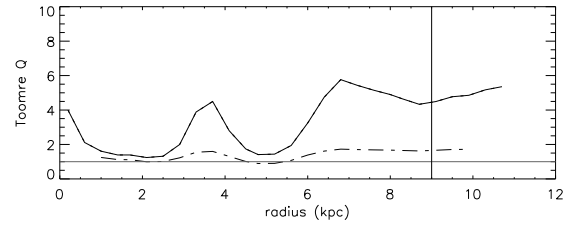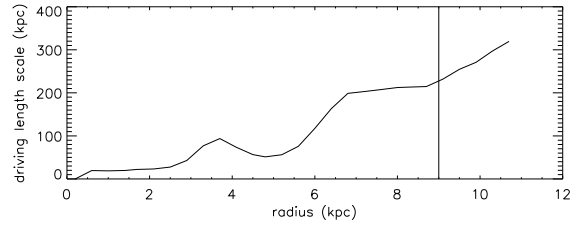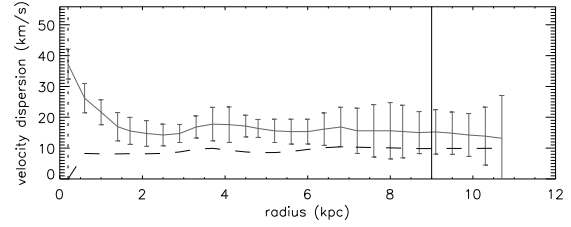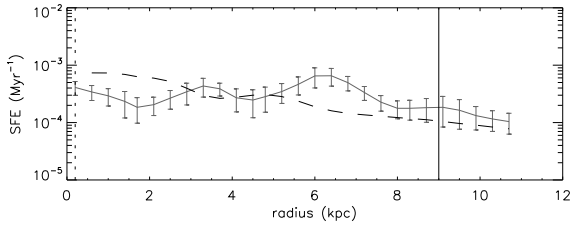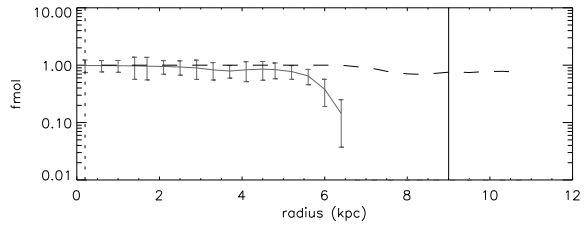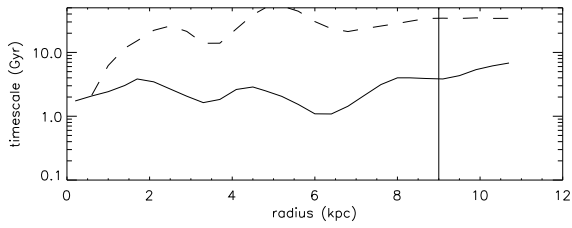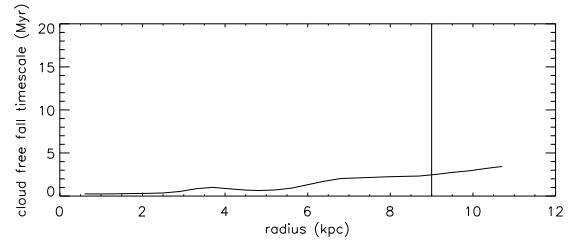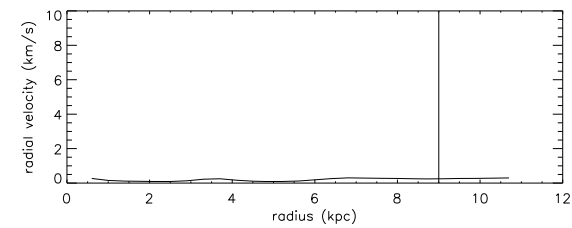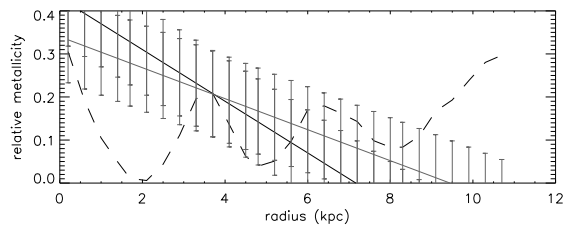

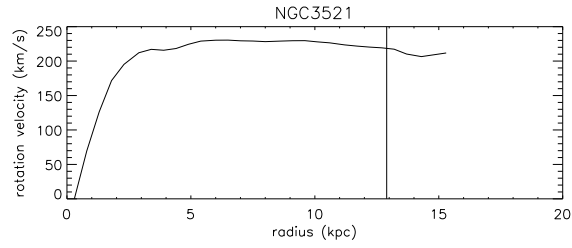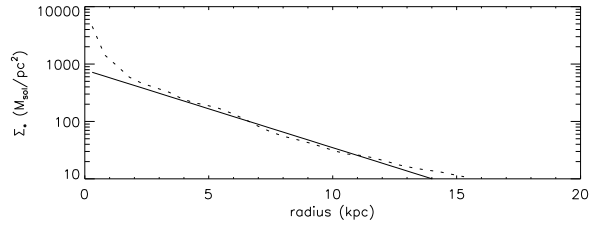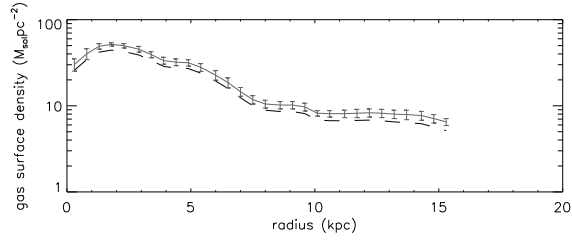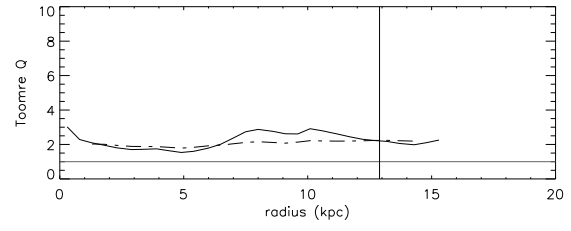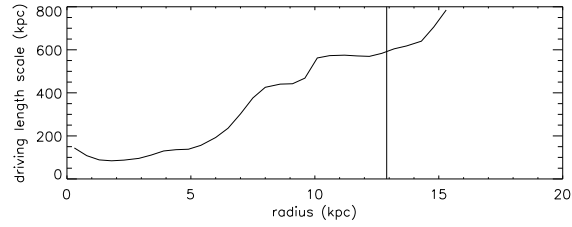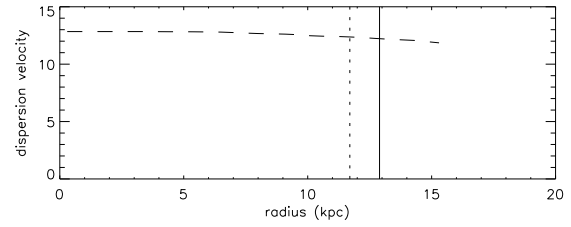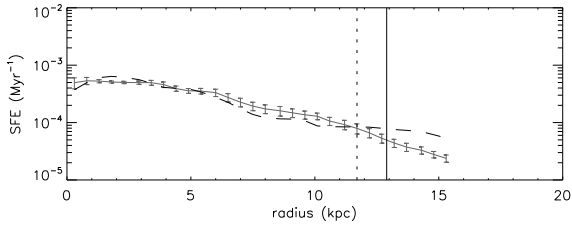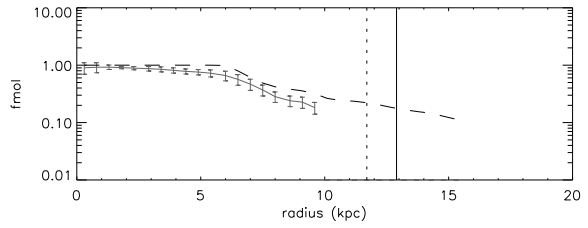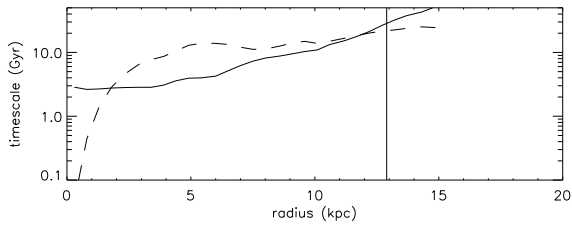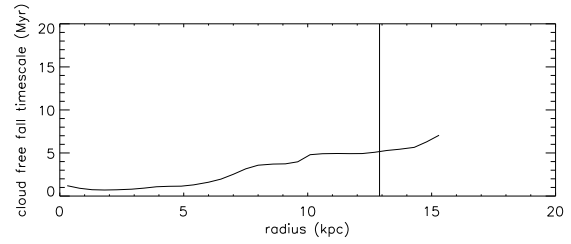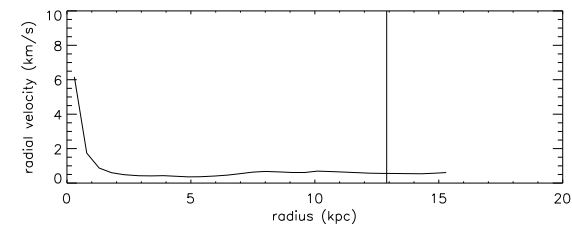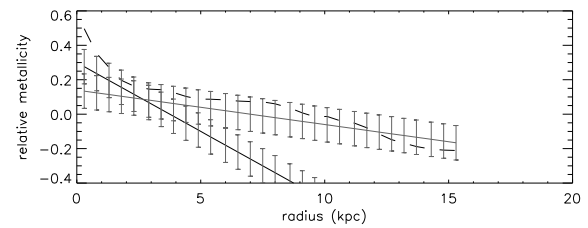

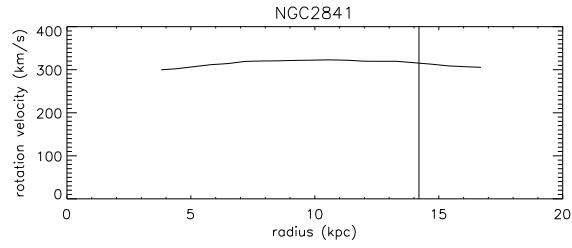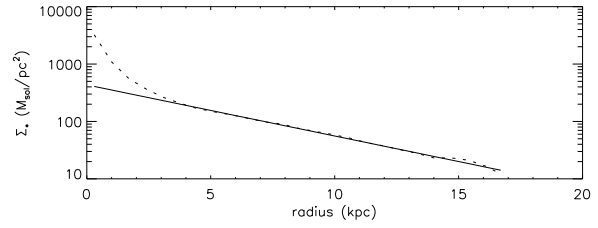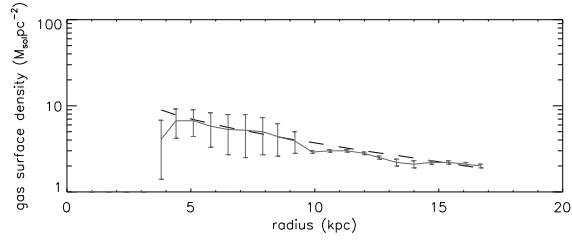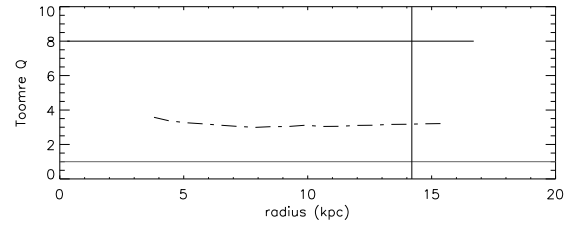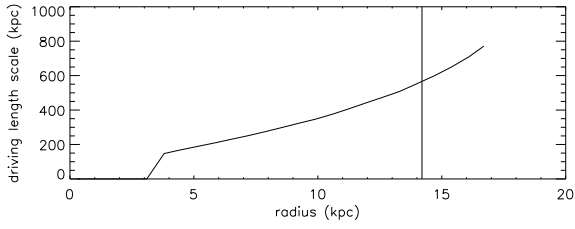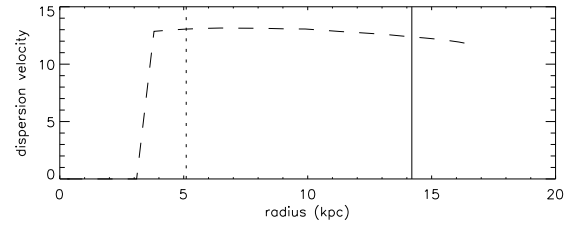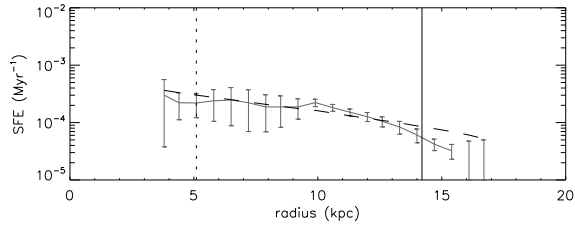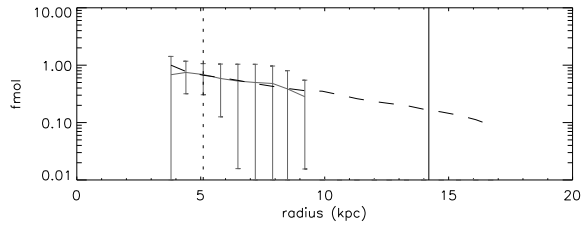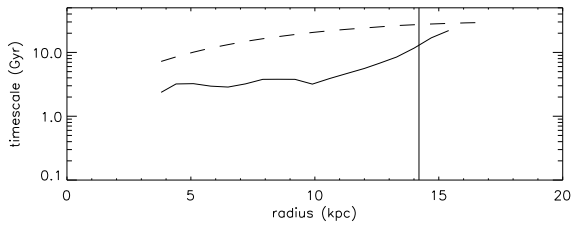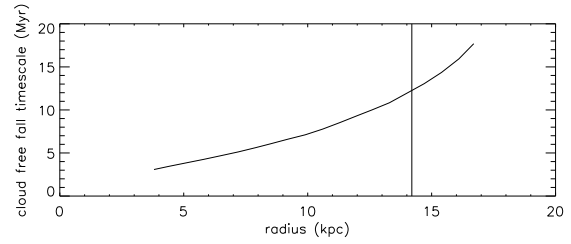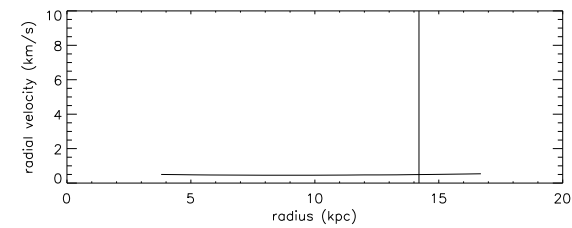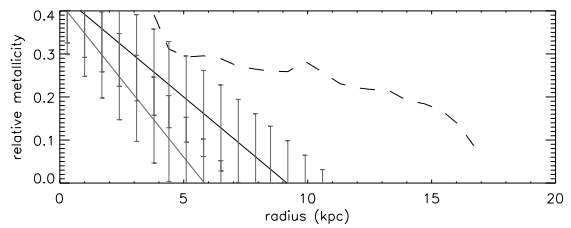



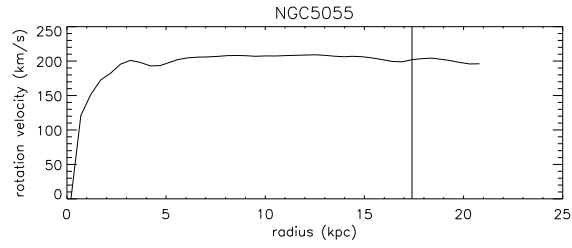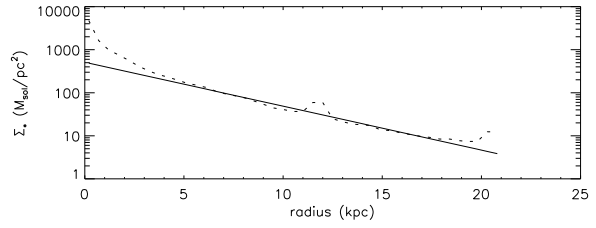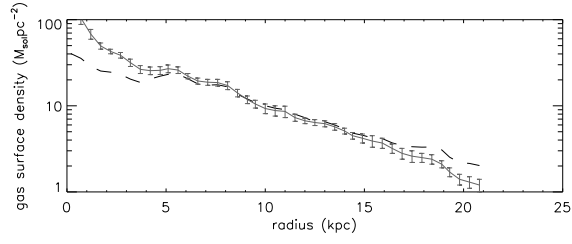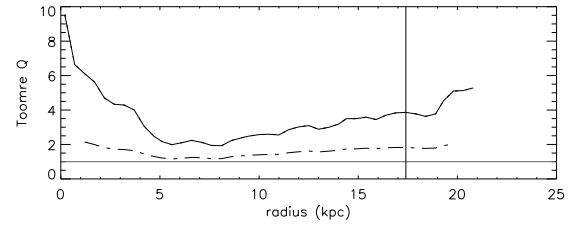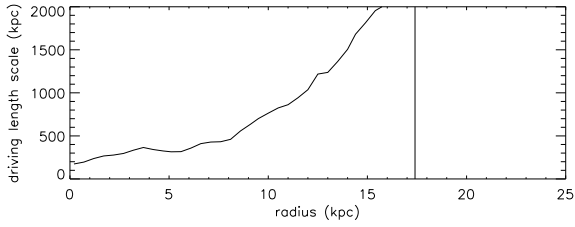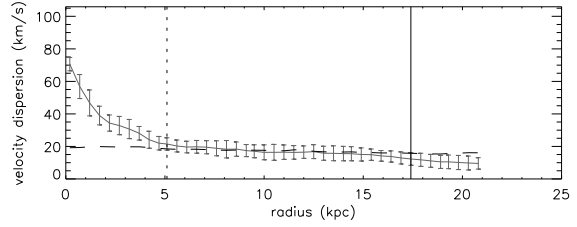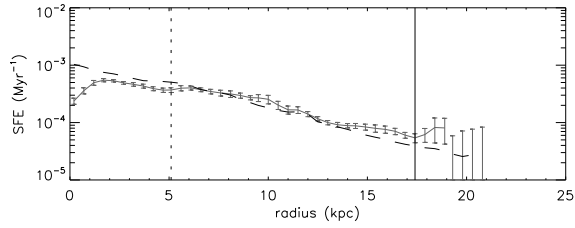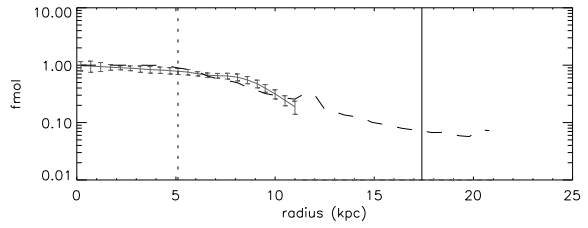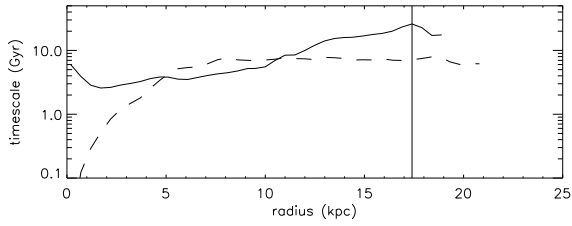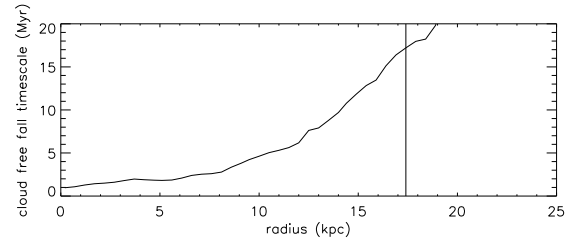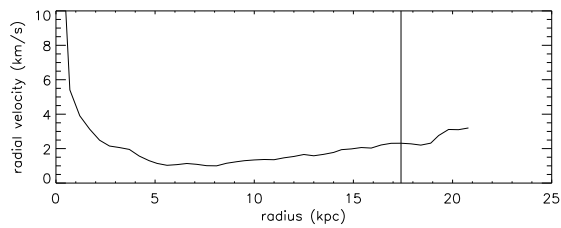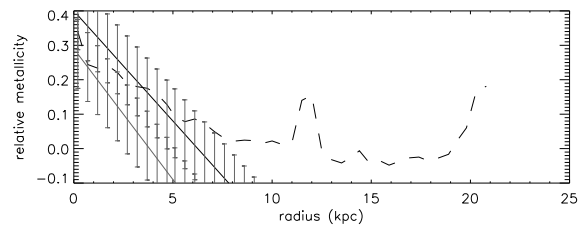

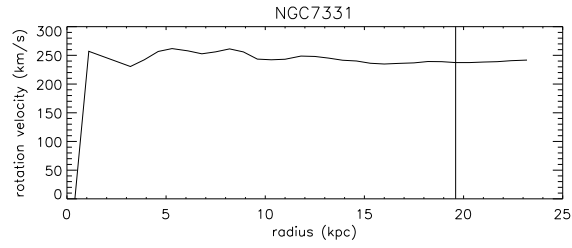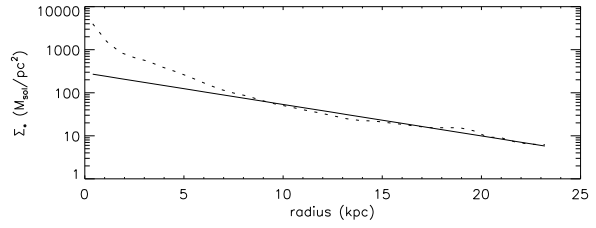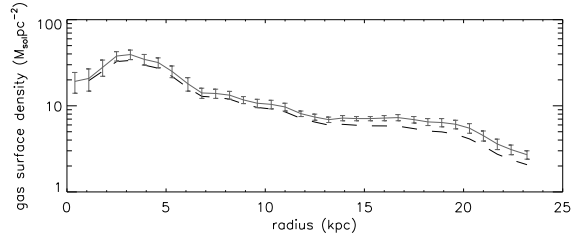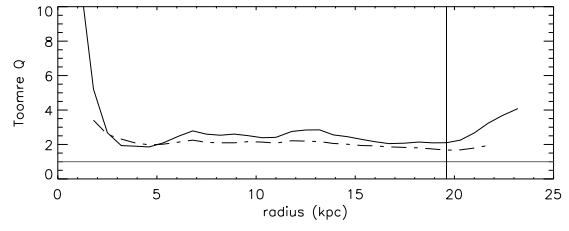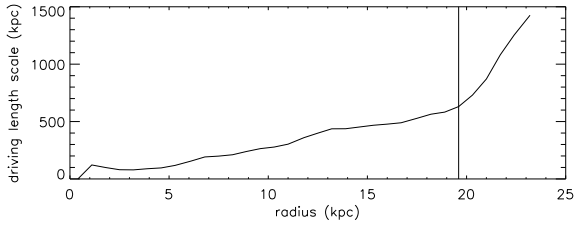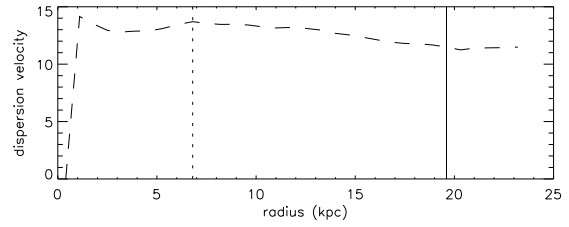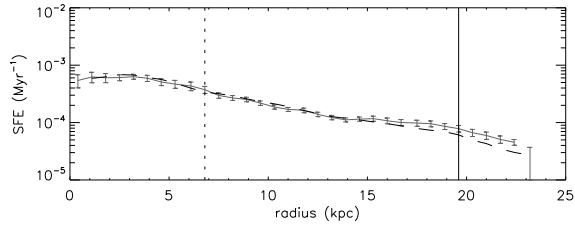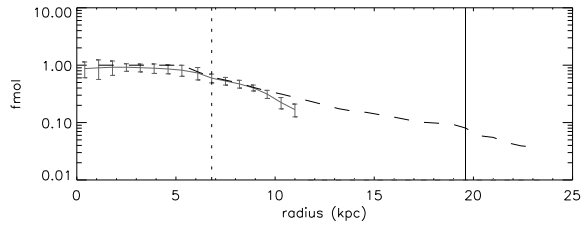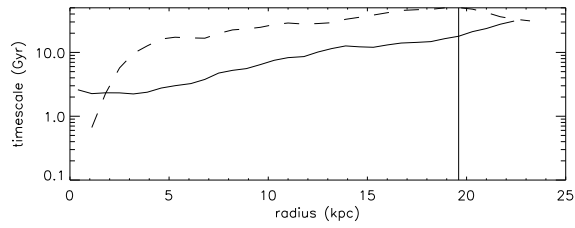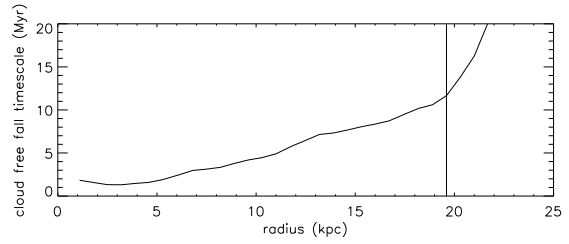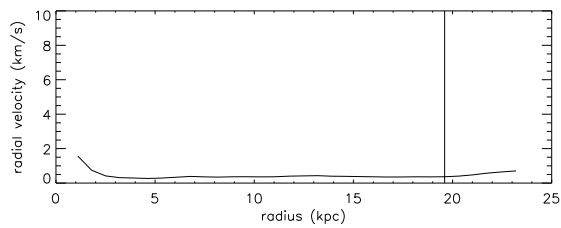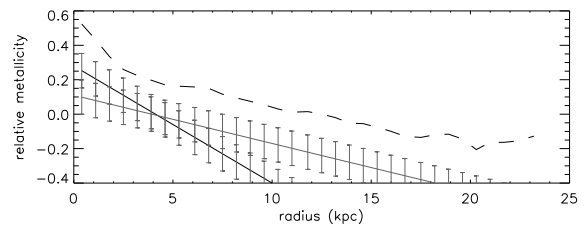

Supplement: Supplementary file 2 [file bvollmer_f2_full.pdf]
